# Supplementary material for: Inference for the panel ARMA-GARCH model when both $N$ and $T$ are large
Source: arXiv:2404.18377 ancillary file (2024-04-29)
Supplement: Supplementary file 1 [file Supplement.pdf]

# Supplementary materials for "Inference for the panel ARMA–GARCH model when both $N$ and $T$ are large"

Bing Su and Ke Zhu*

*University of Hong Kong*

## Appendix A Additional simulation results

In this appendix, some additional simulation results for model (5.1) with student $t$ distributed errors are provided.

Table A.1: Estimation results of bias for model (5.1) with $\epsilon_{it} \overset{i.i.d.}{\sim} \sqrt{0.6}t(5)$.

| | | Bias | | | | | | | | | | | | |
|---|---|---|---|---|---|---|---|---|---|---|---|---|---|---|
| $N$ | $T$ | $\hat{\beta}$ | $\hat{\beta}_A$ | $\hat{\beta}_J$ | $\hat{\phi}$ | $\hat{\phi}_A$ | $\hat{\phi}_J$ | $\hat{\psi}$ | $\hat{\psi}_A$ | $\hat{\psi}_J$ | $\hat{\tau}$ | $\hat{\tau}_J$ | $\hat{\nu}$ | $\hat{\nu}_J$ |
| 50 | 20 | −0.008 | −0.001 | 0.004 | −0.009 | −0.002 | 0.004 | −0.027 | 0.008 | 0.020 | — | — | — | — |
| | 50 | −0.003 | 0.000 | 0.001 | −0.004 | 0.000 | 0.001 | −0.013 | −0.001 | 0.005 | −0.072 | −0.010 | −0.175 | −0.020 |
| | 100 | −0.001 | 0.000 | 0.001 | −0.002 | 0.000 | 0.001 | −0.005 | 0.001 | 0.004 | −0.039 | −0.007 | −0.069 | 0.029 |
| | 200 | −0.001 | 0.000 | 0.000 | −0.001 | 0.000 | 0.000 | −0.003 | 0.000 | 0.001 | −0.021 | −0.004 | −0.028 | 0.013 |
| | 300 | −0.001 | 0.000 | 0.000 | −0.001 | 0.000 | 0.000 | −0.001 | 0.000 | 0.001 | −0.016 | −0.005 | −0.018 | 0.006 |
| 100 | 20 | −0.006 | 0.000 | 0.004 | −0.008 | −0.001 | 0.005 | −0.032 | 0.003 | 0.021 | — | — | — | — |
| | 50 | −0.003 | −0.001 | 0.001 | −0.003 | 0.000 | 0.002 | −0.012 | 0.000 | 0.006 | −0.077 | −0.015 | −0.160 | 0.024 |
| | 100 | −0.002 | 0.000 | 0.001 | −0.002 | 0.000 | 0.000 | −0.005 | 0.000 | 0.003 | −0.040 | −0.007 | −0.070 | 0.023 |
| | 200 | −0.001 | −0.001 | 0.000 | −0.001 | 0.000 | 0.000 | −0.002 | 0.001 | 0.002 | −0.022 | −0.005 | −0.025 | 0.014 |
| | 300 | 0.000 | 0.000 | 0.001 | −0.001 | 0.000 | 0.000 | −0.002 | −0.001 | 0.000 | −0.015 | −0.003 | −0.017 | 0.007 |

*Address correspondence to Department of Statistics & Actuarial Science, University of Hong Kong, Hong Kong, China, E-mail: mazhuke@hku.hk

Table A.2: Estimation results of SD for model (5.1) with $\epsilon_{it} \overset{i.i.d.}{\sim} \sqrt{0.6}t(5)$.

| | | SD | | | | | | | | | | | | |
|---|---|---|---|---|---|---|---|---|---|---|---|---|---|---|
| $N$ | $T$ | $\hat{\beta}$ | $\hat{\beta}_A$ | $\hat{\beta}_J$ | $\hat{\phi}$ | $\hat{\phi}_A$ | $\hat{\phi}_J$ | $\hat{\psi}$ | $\hat{\psi}_A$ | $\hat{\psi}_J$ | $\hat{\tau}$ | $\hat{\tau}_J$ | $\hat{\nu}$ | $\hat{\nu}_J$ |
| 50 | 20 | 0.049 | 0.048 | 0.052 | 0.017 | 0.018 | 0.020 | 0.067 | 0.062 | 0.071 | — | — | — | — |
| | 50 | 0.028 | 0.028 | 0.029 | 0.010 | 0.010 | 0.010 | 0.036 | 0.035 | 0.039 | 0.033 | 0.045 | 0.108 | 0.180 |
| | 100 | 0.021 | 0.021 | 0.021 | 0.007 | 0.007 | 0.008 | 0.025 | 0.024 | 0.026 | 0.026 | 0.032 | 0.080 | 0.108 |
| | 200 | 0.013 | 0.013 | 0.013 | 0.005 | 0.005 | 0.005 | 0.017 | 0.017 | 0.018 | 0.021 | 0.024 | 0.057 | 0.068 |
| | 300 | 0.011 | 0.011 | 0.011 | 0.004 | 0.004 | 0.004 | 0.013 | 0.013 | 0.014 | 0.018 | 0.020 | 0.048 | 0.055 |
| 100 | 20 | 0.034 | 0.033 | 0.036 | 0.013 | 0.013 | 0.015 | 0.046 | 0.042 | 0.048 | — | — | — | — |
| | 50 | 0.020 | 0.020 | 0.021 | 0.008 | 0.008 | 0.008 | 0.025 | 0.025 | 0.027 | 0.023 | 0.032 | 0.083 | 0.141 |
| | 100 | 0.014 | 0.014 | 0.014 | 0.005 | 0.005 | 0.005 | 0.016 | 0.016 | 0.017 | 0.018 | 0.022 | 0.056 | 0.073 |
| | 200 | 0.010 | 0.010 | 0.010 | 0.004 | 0.004 | 0.004 | 0.013 | 0.012 | 0.013 | 0.014 | 0.017 | 0.041 | 0.045 |
| | 300 | 0.008 | 0.008 | 0.008 | 0.003 | 0.003 | 0.003 | 0.011 | 0.011 | 0.011 | 0.013 | 0.015 | 0.033 | 0.036 |

Table A.3: Estimation results of SD/AD for model (5.1) with $\epsilon_{it} \overset{i.i.d.}{\sim} \sqrt{0.6}t(5)$.

| | | SD/AD | | | | | | | | | | | | |
|---|---|---|---|---|---|---|---|---|---|---|---|---|---|---|
| $N$ | $T$ | $\hat{\beta}$ | $\hat{\beta}_A$ | $\hat{\beta}_J$ | $\hat{\phi}$ | $\hat{\phi}_A$ | $\hat{\phi}_J$ | $\hat{\psi}$ | $\hat{\psi}_A$ | $\hat{\psi}_J$ | $\hat{\tau}$ | $\hat{\tau}_J$ | $\hat{\nu}$ | $\hat{\nu}_J$ |
| 50 | 20 | 1.076 | 1.074 | 1.144 | 1.080 | 1.079 | 1.214 | 1.114 | 1.043 | 1.218 | — | — | — | — |
| | 50 | 1.003 | 1.002 | 1.028 | 1.006 | 1.004 | 1.047 | 1.064 | 1.044 | 1.168 | 0.952 | 1.248 | 0.594 | 1.736 |
| | 100 | 1.037 | 1.037 | 1.042 | 1.060 | 1.062 | 1.087 | 1.036 | 1.027 | 1.085 | 0.907 | 1.119 | 0.786 | 1.458 |
| | 200 | 0.935 | 0.935 | 0.939 | 0.990 | 0.990 | 0.997 | 1.020 | 1.016 | 1.057 | 0.890 | 1.040 | 0.855 | 1.185 |
| | 300 | 0.992 | 0.992 | 0.996 | 1.035 | 1.035 | 1.038 | 0.981 | 0.979 | 1.004 | 0.894 | 1.017 | 0.905 | 1.124 |
| 100 | 20 | 1.052 | 1.041 | 1.130 | 1.122 | 1.101 | 1.299 | 1.041 | 0.975 | 1.136 | — | — | — | — |
| | 50 | 1.030 | 1.029 | 1.044 | 1.105 | 1.105 | 1.152 | 1.028 | 1.007 | 1.117 | 0.959 | 1.253 | 0.638 | 1.976 |
| | 100 | 0.976 | 0.975 | 0.981 | 1.057 | 1.056 | 1.078 | 0.953 | 0.944 | 1.002 | 0.861 | 1.062 | 0.769 | 1.383 |
| | 200 | 1.017 | 1.017 | 1.019 | 1.036 | 1.035 | 1.041 | 1.007 | 1.002 | 1.027 | 0.889 | 1.041 | 0.869 | 1.156 |
| | 300 | 1.035 | 1.035 | 1.033 | 1.028 | 1.028 | 1.022 | 1.028 | 1.025 | 1.045 | 0.912 | 1.064 | 0.891 | 1.101 |

# Appendix B Expressions

In this appendix, we first give the expressions of $\partial\hat{Q}_\lambda/\partial\lambda$, $\hat{D}$, $D$, $\mathrm{E}(D)$, $\partial^2\hat{Q}_\lambda/\partial\lambda\partial\lambda'$, $\hat{S}$, $S$, $\mathrm{E}(S)$, $\Omega_1$ and $\mathrm{E}(D^\dagger)$ for the panel ARMA specification. Second, we provide the explicit formulas of $\partial L_{\zeta,\omega}/\partial\zeta$, $\partial^2 L_{\zeta,\omega}/\partial\zeta\partial\zeta'$, $\mathcal{O}^\sharp_{23,it}$, and $\Pi$ for the panel GARCH specification. For ease of presentation, the explicit formulas of $\Delta^\S$, $\Delta^\sharp$, and $\Delta^\flat$ are deferred in (C.46), (C.55), and (C.62) below, respectively.

## B.1 Expressions for the panel ARMA specification

For a matrix $M_\theta$, we rewrite $M_{\theta_0}$ as $M_0$ or $M$ for simplicity. For example, $A_{\phi_0}$, $B_{\psi_0}$, $\Sigma_{\psi_0}$, and $C_{\psi_0}$ are denoted as $A$, $B$, $\Sigma$, and $C$, respectively.

First, the first derivative $\partial\hat{Q}_\lambda/\partial\lambda$ is given by

$$\frac{\partial\hat{Q}_\lambda}{\partial\beta} = -2V'_{\phi,\beta}(I_N\otimes(\Sigma_\psi^{-1}-C_\psi))X,$$
$$\frac{\partial\hat{Q}_\lambda}{\partial\phi_p} = 2V'_{\phi,\beta}(I_N\otimes(\Sigma_\psi^{-1}-C_\psi)\dot{A}_p)Y,$$
$$\frac{\partial\hat{Q}_\lambda}{\partial\psi_q} = V'_{\phi,\beta}(I_N\otimes H_q)V_{\phi,\beta},$$

where $\dot{A}_p=\partial A_\phi/\partial\phi_p$ and $H_q = 2\Sigma_\psi^{-1}\dot{\Sigma}_q C_\psi - \Sigma_\psi^{-1}\dot{\Sigma}_q\Sigma_\psi^{-1} - \mathrm{tr}(\dot{\Sigma}_q C_\psi)C_\psi$ with $\dot{\Sigma}_q=\partial\Sigma_\psi/\partial\psi_q$. By using the fact $V_{\phi,\beta}=(I_N\otimes B_\psi)\hat{U}_{\theta_1}+(I_N\otimes l_T)\mu$, it follows that $\hat{D}=\partial\hat{Q}_\lambda/\partial\lambda\big|_{\theta_1=\theta_{01}} = ((\hat{D}^\beta)',\hat{D}^{\phi_1},...,\hat{D}^{\phi_P},\hat{D}^{\psi_1},...,\hat{D}^{\psi_Q})'$, where

$$\hat{D}^\beta = \frac{\partial\hat{Q}_\lambda}{\partial\beta}\Big|_{\theta_1=\theta_{01}} = -2\hat{U}'_{\theta_{01}}(I_N\otimes B'(\Sigma^{-1}-C))X,$$
$$\hat{D}^{\phi_p} = \frac{\partial\hat{Q}_\lambda}{\partial\phi_p}\Big|_{\theta_1=\theta_{01}} = 2\hat{U}'_{\theta_{01}}(I_N\otimes B'A^*_{0p}B)\hat{U}_{\theta_{01}} + 2\hat{U}'_{\theta_{01}}(I_N\otimes B'A^*_{0p})((I_N\otimes l_T)\mu_0+X\beta_0),$$
$$\hat{D}^{\psi_q} = \frac{\partial\hat{Q}_\lambda}{\partial\psi_q}\Big|_{\theta_1=\theta_{01}} = \hat{U}'_{\theta_{01}}(I_N\otimes B'H_{0q}B)\hat{U}_{\theta_{01}} + 2\hat{U}'_{\theta_{01}}(I_N\otimes B'H_{0q}l_T)\mu_0,$$

where $A^*_p=(\Sigma_\psi^{-1}-C_\psi)\dot{A}_pA_\phi^{-1}$. By replacing $\hat{U}_{\theta_{01}}$ in $\hat{D}$ with $U$, we can show that $D=((D^\beta)',D^{\phi_1},...,D^{\phi_P},D^{\psi_1},...,D^{\psi_Q})'$, where

$$D^\beta = -2U'(I_N\otimes B'(\Sigma^{-1}-C))X,$$
$$D^{\phi_p} = 2U'(I_N\otimes B'A^*_{0p}B_\psi)U + 2U'(I_N\otimes B'A^*_{0p})((I_N\otimes l_T)\mu_0+X\beta_0), \tag{B.1}$$
$$D^{\psi_q} = U'(I_N\otimes B'H_{0q}B)U + 2U'(I_N\otimes B'H_{0q}l_T)\mu_0.$$

Then, $\mathrm{E}(D)$ can be computed as

$$\begin{aligned} &\mathrm{E}(D^{\beta}) = 0, \qquad \mathrm{E}(D^{\phi_p}) = -2\mathrm{tr}\big(\mathrm{diag}(\omega_0) \otimes B'C\dot{A}_{0p}A^{-1}B\big), \\ &\mathrm{E}(D^{\psi_q}) = 2\mathrm{tr}\big(\mathrm{diag}(\omega_0) \otimes B'\Sigma^{-1}\dot{\Sigma}_{0q}CB\big) - \mathrm{tr}(\dot{\Sigma}_{0q}C)\mathrm{tr}\big(\mathrm{diag}(\omega_0) \otimes B'CB\big). \end{aligned} \tag{B.2}$$

Next, the second derivative $\partial^2\hat{Q}_\lambda/\partial\lambda\partial\lambda'$ is given by

$$\begin{aligned} &\frac{\partial^2\hat{Q}_\lambda}{\partial\beta\partial\beta'} = 2X'(I_N \otimes (\Sigma_\psi^{-1} - C_\psi))X, \quad &&\frac{\partial^2\hat{Q}_\lambda}{\partial\beta\partial\phi_p} = -2Y'(I_N \otimes \dot{A}_p'(\Sigma_\psi^{-1} - C_\psi))X, \\ &\frac{\partial^2\hat{Q}_\lambda}{\partial\beta\partial\psi_q} = -2V_{\phi,\beta}'(I_N \otimes H_q)X, &&\frac{\partial^2\hat{Q}_\lambda}{\partial\phi_p\partial\phi_{p^*}} = 2Y'(I_N \otimes \dot{A}_{p^*}'(\Sigma_\psi^{-1} - C_\psi)\dot{A}_p)Y, \\ &\frac{\partial^2\hat{Q}_\lambda}{\partial\phi_p\partial\psi_q} = 2V_{\phi,\beta}'(I_N \otimes H_q\dot{A}_p)Y, &&\frac{\partial^2\hat{Q}_\lambda}{\partial\psi_q\partial\psi_{q^*}} = V_{\phi,\beta}'(I_N \otimes E_{qq^*})V_{\phi,\beta}, \end{aligned} \tag{B.3}$$

where $E_{qq^*} = 2\Sigma_\psi^{-1}\dot{\Sigma}_{q^*}\Sigma_\psi^{-1}\dot{\Sigma}_q\Sigma_\psi^{-1} - \Sigma_\psi^{-1}\ddot{\Sigma}_{qq^*}\Sigma_\psi^{-1} - \mathrm{tr}(\ddot{\Sigma}_{qq^*}C_\psi)C_\psi - 2\big[\mathrm{tr}(\dot{\Sigma}_qC_\psi)\mathrm{tr}(\dot{\Sigma}_{q^*}C_\psi) - \mathrm{tr}(\dot{\Sigma}_q\Sigma_\psi^{-1}\dot{\Sigma}_{q^*}C_\psi) - \mathrm{tr}(\dot{\Sigma}_qC_\psi)\Sigma_\psi^{-1}\dot{\Sigma}_{q^*} + \Sigma_\psi^{-1}\dot{\Sigma}_{q^*}\Sigma_\psi^{-1}\dot{\Sigma}_q - \Sigma_\psi^{-1}\ddot{\Sigma}_{qq^*} + 2\Sigma_\psi^{-1}\dot{\Sigma}_q\Sigma_\psi^{-1}\dot{\Sigma}_{q^*} - \mathrm{tr}(\dot{\Sigma}_{q^*}C_\psi)\Sigma_\psi^{-1}\dot{\Sigma}_q\big]C_\psi$ with $\ddot{\Sigma}_{qq^*} = \partial^2\Sigma_\psi/\partial\psi_q\partial\psi_{q^*}$. Now, we can define $\hat{S} = \partial^2\hat{Q}_\lambda/\partial\lambda\partial\lambda'\big|_{\lambda=\lambda_0}$ and $S$, where $S$ is defined in the same way as $\hat{S}$, with $\hat{U}_{\theta_{01}}$ replaced by $U$. Then, $\mathrm{E}(S)$ can be computed as

$$\begin{aligned} \mathrm{E}(S^{\beta\beta'}) &= 2\mathrm{E}\big(X'(I_N \otimes (\Sigma^{-1} - C))X\big), \\ \mathrm{E}(S^{\beta\phi_p}) &= -2\mathrm{E}\big((X\beta_0 + \mu_0 \otimes l_T)'(I_N \otimes A^{-1'}\dot{A}_{0p}'(\Sigma^{-1} - C))X\big), \\ \mathrm{E}(S^{\beta\psi_q}) &= -2(\mu_0' \otimes l_T'H_{0q})\mathrm{E}(X), \\ \mathrm{E}(S^{\phi_p\phi_{p^*}}) &= 2\mathrm{E}\big((X\beta_0 + \mu_0 \otimes l_T)'(I_N \otimes M_{0pp^*})(X\beta_0 + \mu_0 \otimes l_T)\big) \\ &\qquad + 2\mathrm{tr}(\mathrm{diag}(\omega_0) \otimes B'M_{0,pp^*}B), \\ \mathrm{E}(S^{\phi_p\psi_q}) &= 2(\mu_0' \otimes l_T'H_{0q}\dot{A}_{0p}A^{-1})(\mathrm{E}(X)\beta_0 + \mu_0 \otimes l_T) \\ &\qquad + 2\mathrm{tr}(\mathrm{diag}(\omega_0) \otimes B'H_{0q}\dot{A}_{0p}A^{-1}B), \\ \mathrm{E}(S^{\psi_q\psi_{q^*}}) &= (\mu_0'\mu_0)(l_T'E_{0qq^*}l_T) + \mathrm{tr}(\mathrm{diag}(\omega_0) \otimes B'E_{0qq^*}B), \end{aligned} \tag{B.4}$$

where $M_{pp^*} = A_\phi^{-1'}\dot{A}_{p^*}'(\Sigma_\psi^{-1} - C_\psi)\dot{A}_pA_\phi^{-1}$. Note that $S^{\beta\phi_p}$ is $\partial^2\hat{Q}_\lambda/\partial\beta\partial\phi_p\big|_{\lambda=\lambda_0}$ with $\hat{U}_{\theta_{01}}$ replaced by $U$, and the other items in (B.4) are defined similarly. Clearly, under (B.4), the formula of $\Gamma_1 = -(NT)^{-1}\mathrm{E}(S)$ follows directly.

Moreover, we focus on the expression for $\Omega_1 = (NT)^{-1}\mathrm{E}\{[D - \mathrm{E}(D)][D - \mathrm{E}(D)]'\}$. Denote two linear-quadratic forms $\mathcal{LQ}^{(1)} = V'M^{(1)}V + b^{(1)'}V$ and $\mathcal{LQ}^{(2)} = V'M^{(2)}V +$

$b^{(2)\prime}V$, where $M^{(1)}$, $M^{(2)}$, $b^{(1)}$, and $b^{(2)}$ are defined as $M$ and $b$ in (3.1). Like (C.1)–(C.2) below, we can show

$$\begin{aligned}
&\mathrm{E}\{[\mathcal{LQ}^{(1)} - \mathrm{E}(\mathcal{LQ}^{(1)})][\mathcal{LQ}^{(2)} - \mathrm{E}(\mathcal{LQ}^{(2)})]'\} \\
&= \sum_{i=1}^{N}\sum_{t=1}^{T}(\varrho_i - 3\sigma_i^4)m_{ii,tt}^{(1)}m_{ii,tt}^{(2)} + \sum_{i=1}^{N}\sum_{t=1}^{T}\Big[a_{it}^{(**)} + e_{it}^{(12)} + e_{it}^{(21)} + f_{it}^{(12)} + f_{it}^{(21)} \\
&\quad + g_{it}^{(12)} + g_{it}^{(21)} + \pi_i b_{it}^{(1)} m_{ii,tt}^{(2)} + \pi_i b_{it}^{(2)} m_{ii,tt}^{(1)}\Big] \\
&\quad + \sum_{i=1}^{N}\sum_{j=1}^{N}\sigma_i^2\sigma_j^2\left[\mathrm{tr}(M_{ij}^{(1)}M_{ij}^{(2)\prime}) + \mathrm{tr}(M_{ij}^{(1)}M_{ji}^{(2)})\right] + \sum_{i=1}^{N}\sigma_i^2 b_i^{(1)\prime} b_i^{(2)},
\end{aligned} \tag{B.5}$$

where

$$\begin{aligned}
a_{it}^{**} &= \sum\nolimits_{t^*=1,t^*\neq t}^{T}\left[m_{ii,tt}^{(1)}m_{ii,t^*t^*}^{(2)} + m_{ii,tt^*}^{(1)}m_{ii,tt^*}^{(2)} + m_{ii,tt^*}^{(1)}m_{ii,t^*t}^{(2)}\right]\varsigma_{i,t,t^*}, \\
e_{it}^{(12)} &= \sum\nolimits_{t^*=1,t^*\neq t}^{T}\sum\nolimits_{t^\sharp=1,t^\sharp\neq t,t^*}^{T}\Big[m_{ii,tt}^{(1)}m_{ii,t^*t^\sharp}^{(2)} + m_{ii,tt^*}^{(1)}m_{ii,tt^\sharp}^{(2)} + m_{ii,tt^*}^{(1)}m_{ii,t^\sharp t}^{(2)} \\
&\qquad\qquad + m_{ii,t^*t}^{(1)}m_{ii,t^\sharp t}^{(2)} + m_{ii,t^*t}^{(1)}m_{ii,tt^\sharp}^{(2)}\Big]\vartheta_{i,t,t^*,t^\sharp}, \\
f_{it}^{(12)} &= \sum\nolimits_{t^*=1,t^*\neq t}^{T}\left[m_{ii,tt}^{(1)}m_{ii,tt^*}^{(2)} + m_{ii,tt}^{(1)}m_{ii,t^*t}^{(2)}\right]\varrho_{i,t,t^*}, \\
g_{it}^{(12)} &= \sum\nolimits_{t^*=1,t^*\neq t}^{T}\left[m_{ii,tt}^{(1)}b_{it^*}^{(2)} + m_{ii,tt^*}^{(1)}b_{it}^{(2)} + m_{ii,t^*t}^{(1)}b_{it}^{(2)}\right]\pi_{i,t,t^*},
\end{aligned}$$

and $e_{it}^{(21)}$, $f_{it}^{(21)}$, and $g_{it}^{(21)}$ are defined similarly. If $M^{(1)} = M^{(2)}$ and $b^{(1)} = b^{(2)}$, (B.5) reduces to the formula of $\sigma_{\mathcal{LQ}}^2$. As shown in (B.1), $D$ has the linear-quadratic structure as $\mathcal{LQ}$[1]. Consequently, the explicit formula of $\Omega_1$ can be provided, since according to (B.1), all terms in $\mathrm{E}\{[D - \mathrm{E}(D)][D - \mathrm{E}(D)]'\}$ have the structure as in (B.5).

Finally, we show how to write down the explicit formula of $\mathrm{E}(D^\dagger) = \mathrm{E}(\hat{D} - D)$. By (B.1), it is observed that $D^\dagger$ has the same structure as $\mathcal{LQ}^\dagger$ in Lemma C.2 below. Note that the expressions for $\mathrm{E}(\mathcal{LQ}^\dagger)$ are given in (C.11) and (C.13) below for the ARMA$(1,1)$ and ARMA$(P,Q)$ cases, respectively. From these expressions, we can give the formula of $\mathrm{E}(D^\dagger)$ straightforwardly. Particularly, it is not difficult to check that when $Q = 0$ (i.e., $\psi_{0q} = 0$), $\mathrm{E}(D^\dagger)$ becomes zero.

## B.2 Expressions for the panel GARCH specification

Without loss of generality (w.l.o.g.), we suppose that $K = L$, and denote that $\kappa_k = \tau_k + \nu_k$. Note that the undefined parameters are set to be zero, i.e., $\nu_k = 0$ when $K < k \leq L$.

[1]For example, $D^{\psi_q}$ can be rewritten as $U'M^{\psi_q}U + (b^{\psi_q})'U$ with $M^{\psi_q} = I_N \otimes B'H_{0q}B$ and $2\mu_0'(I_N \otimes l_T'H_{0q}'B)$.

First, by (2.8), the first derivative $\partial L_{\zeta,\omega}/\partial\zeta$ is given by

$$\begin{aligned}\frac{\partial L_{\zeta,\omega}}{\partial\tau_l} &= \frac{1}{2}\sum_{i=1}^{N}\sum_{t=1}^{T}\frac{u_{it}^2 - h_{it,\zeta,\omega_i}}{h_{it,\zeta,\omega_i}^2}\frac{\partial h_{it,\zeta,\omega_i}}{\partial\tau_l},\\ \frac{\partial L_{\zeta,\omega}}{\partial\nu_k} &= \frac{1}{2}\sum_{i=1}^{N}\sum_{t=1}^{T}\frac{u_{it}^2 - h_{it,\zeta,\omega_i}}{h_{it,\zeta,\omega_i}^2}\frac{\partial h_{it,\zeta,\omega_i}}{\partial\nu_k}.\end{aligned} \tag{B.6}$$

Then, $\hat{G} = \partial\hat{L}_{\zeta,\hat{\omega}}/\partial\zeta\big|_{\zeta=\zeta_0}$ with its variations $\check{G}$, $\tilde{G}$, $\bar{G}$, and $G$ can be obtained according to (4.5)–(4.8).

Next, the second derivative $\partial^2 L_{\zeta,\omega}/\partial\zeta\partial\zeta'$ consists of

$$\frac{\partial^2 L_{\zeta,\omega}}{\partial\tau_l\partial\tau_{l^*}} = -\frac{1}{2}\sum_{i=1}^{N}\sum_{t=1}^{T}\frac{2u_{it}^2 - h_{it,\zeta,\omega_i}}{h_{it,\zeta,\omega_i}^3}\frac{\partial h_{it,\zeta,\omega_i}}{\partial\tau_l}\frac{\partial h_{it,\zeta,\omega_i}}{\partial\tau_{l^*}},$$

$$\frac{\partial^2 L_{\zeta,\omega}}{\partial\nu_k\partial\nu_{k^*}} = -\frac{1}{2}\sum_{i=1}^{N}\sum_{t=1}^{T}\frac{2u_{it}^2 - h_{it,\zeta,\omega_i}}{h_{it,\zeta,\omega_i}^3}\frac{\partial h_{it,\zeta,\omega_i}}{\partial\nu_k}\frac{\partial h_{it,\zeta,\omega_i}}{\partial\nu_{k^*}},$$

$$\frac{\partial^2 L_{\zeta,\omega}}{\partial\tau_l\partial\nu_k} = -\frac{1}{2}\sum_{i=1}^{N}\sum_{t=1}^{T}\frac{2u_{it}^2 - h_{it,\zeta,\omega_i}}{h_{it,\zeta,\omega_i}^3}\frac{\partial h_{it,\zeta,\omega_i}}{\partial\tau_l}\frac{\partial h_{it,\zeta,\omega_i}}{\partial\nu_k} + \frac{1}{2}\sum_{i=1}^{N}\sum_{t=1}^{T}\frac{u_{it}^2 - h_{it,\zeta,\omega_i}}{h_{it,\zeta,\omega_i}^2}\frac{\partial^2 h_{it,\zeta,\omega_i}}{\partial\tau_l\partial\nu_k},$$

where $\partial h_{it,\zeta,\omega_i}/\partial\tau_l$, $\partial h_{it,\zeta,\omega_i}/\partial\nu_k$ and $\partial^2 h_{it,\zeta,\omega_i}/\partial\tau_l\partial\nu_k$ satisfy

$$\begin{aligned}\frac{\partial h_{it,\zeta,\omega_i}}{\partial\tau_l} &= -\omega_i + u_{i,t-l}^2 + \sum_{k=1}^{K}\nu_k\frac{\partial h_{i,t-k,\zeta,\omega_i}}{\partial\tau_l},\\ \frac{\partial h_{it,\zeta,\omega_i}}{\partial\nu_k} &= -\omega_i + h_{i,t-k,\zeta,\omega_i} + \sum_{k^*=1}^{K}\nu_{k^*}\frac{\partial h_{i,t-k^*,\zeta,\omega_i}}{\partial\nu_k},\\ \frac{\partial^2 h_{it,\zeta,\omega_i}}{\partial\tau_l\partial\nu_k} &= \frac{\partial h_{i,t-k,\zeta,\omega_i}}{\partial\tau_l} + \sum_{k^*=1}^{K}\nu_{k^*}\frac{\partial^2 h_{i,t-k^*,\zeta,\omega_i}}{\partial\tau_l\partial\nu_k}.\end{aligned} \tag{B.7}$$

By (2.7), we have

$$h_{it,\zeta,\omega_i} = \omega_i\Big(1 - \sum_{k=1}^{K}\nu_k\Big)^{-1}\Big(1 - \sum_{l=1}^{L}\kappa_l\Big) + \Big(1 - \sum_{k=1}^{K}\nu_k\mathcal{B}^k\Big)^{-1}\Big(\sum_{l=1}^{L}\tau_l\mathcal{B}^l\Big)u_{it}^2, \tag{B.8}$$

where $\mathcal{B}$ is the back-shift operator satisfying $\mathcal{B}u_{it}^2 = u_{i,t-1}^2$. It follows that

$$\begin{aligned}\frac{\partial h_{it,\zeta,\omega_i}}{\partial\tau_l} &= \Big(1 - \sum_{k=1}^{K}\nu_k\mathcal{B}^k\Big)^{-1}\mathcal{B}^l(u_{it}^2 - \omega_i),\\ \frac{\partial h_{it,\zeta,\omega_i}}{\partial\nu_k} &= \Big(1 - \sum_{k^*=1}^{K}\nu_{k^*}\mathcal{B}^{k^*}\Big)^{-2}\Big(\sum_{l=1}^{L}\tau_l\mathcal{B}^{l+k}\Big)(u_{it}^2 - \omega_i),\\ \frac{\partial^2 h_{it,\zeta,\omega_i}}{\partial\tau_l\partial\nu_k} &= \Big(1 - \sum_{k^*=1}^{K}\nu_{k^*}\mathcal{B}^{k^*}\Big)^{-2}\mathcal{B}^{l+k}(u_{it}^2 - \omega_i).\end{aligned} \tag{B.9}$$

Note that (B.7) and (B.9) are equivalent. The former is convenient for computation, while the latter is convenient for the asymptotic analysis.

Finally, we define $\mathcal{O}^{\sharp}_{23,it}$ and $\Pi$ as follows:

$$\mathcal{O}^{\sharp}_{23,it} = -\frac{2}{h_{it}^2}\Big[\Big(1-\sum_{k=1}^{K}\nu_{0k}\mathcal{B}^k\Big)^{-1}\Big(1-\sum_{k=1}^{K}\kappa_{0k}\mathcal{B}^k\Big)u_{it}\Big]\frac{\partial h_{it}}{\partial \zeta}, \tag{B.10}$$

$$\Pi = \frac{1}{2N}\sum_{i=1}^{N}\mathrm{E}\Big[\frac{1}{h_{it}^2}\frac{\partial h_{it}}{\partial \zeta}\pi^*_{it}\Big], \tag{B.11}$$

where $\pi^*_{it} = ((\pi^{*\beta}_{it})', \pi^{*\phi_1}_{it}, ..., \pi^{*\phi_P}_{it}, \pi^{*\psi_1}_{it}, ..., \pi^{*\psi_Q}_{it})'$ with

$$\pi^{*\beta}_{it} = \Big[\big(1-\sum_{k=1}^{K}\nu_{0k}\mathcal{B}^k\big)^{-1}\big(\sum_{l=1}^{L}\tau_{0l}\mathcal{B}^l\big)2u_{it}\Big]\Big[\big(1+\sum_{q=1}^{Q}\psi_{0q}\mathcal{B}^q\big)(x_{it}-\mathrm{E}(x_{it}))\Big],$$

$$\pi^{*\phi_p}_{it} = \Big[\big(1-\sum_{k=1}^{K}\nu_{0k}\mathcal{B}^k\big)^{-1}\big(\sum_{l=1}^{L}\tau_{0l}\mathcal{B}^l\big)2u_{it}\Big]\Big[\big(1+\sum_{q=1}^{Q}\psi_{0q}\mathcal{B}^q\big)(y_{i,t-p}-\mathrm{E}(y_{i,t-p}))\Big],$$

$$\pi^{*\psi_q}_{it} = \Big[\big(1-\sum_{k=1}^{K}\nu_{0k}\mathcal{B}^k\big)^{-1}\big(\sum_{l=1}^{L}\tau_{0l}\mathcal{B}^l\big)2u_{it}\Big]\Big[\big(1+\sum_{q=1}^{Q}\psi_{0q}\mathcal{B}^q\big)u_{i,t-q}\Big].$$

# Appendix C Proofs

This appendix provides the proofs for linear-quadratic form, panel ARMA specification, and panel GARCH specification in Sections 3–4. For simplicity, the letters $c$ and $c^*$ denote generic constants, whose values can vary along the text.

## C.1 Proofs for linear-quadratic form

**Proof for Theorem 3.1.** Under Condition 2, it is straightforward to show

$$\mathrm{E}(V'MV)^2 = \mathcal{M}_1 + \mathcal{M}_2 + \mathcal{M}_3 + \mathcal{M}_4,$$

where

$$\mathcal{M}_1 = \sum_{i=1}^{N}\mathrm{E}(v_i'M_{ii}v_i)^2 = \sum_{i=1}^{N}\sum_{t=1}^{T}(\mu_{i,4}-3\sigma_i^4)m_{ii,tt}^2 + \sum_{i=1}^{N}\sum_{t=1}^{T}(a_{it}+2e_{it}+2f_{it}) + \sum_{i=1}^{N}c_{m,i},$$

$$\mathcal{M}_2 = \sum_{i=1}^{N}\sum_{j=1,j\neq i}^{N}\mathrm{E}(v_i'M_{ii}v_i)\mathrm{E}(v_j'M_{jj}v_j) = \sum_{i=1}^{N}\sum_{j=1,j\neq i}^{N}\sigma_i^2\sigma_j^2\mathrm{tr}(M_{ii})\mathrm{tr}(M_{jj}),$$

$$\mathcal{M}_3 = \sum_{i=1}^{N}\sum_{j=1,j\neq i}^{N} \mathrm{E}(v_i' M_{ij} v_j)^2 = \sum_{i=1}^{N}\sum_{j=1,j\neq i}^{N} \sigma_i^2\sigma_j^2 \mathrm{tr}(M_{ij}M_{ij}'),$$

$$\mathcal{M}_4 = \sum_{i=1}^{N}\sum_{j=1,j\neq i}^{N} \mathrm{E}(v_i' M_{ij} v_j)(v_j' M_{ji} v_i) = \sum_{i=1}^{N}\sum_{j=1,j\neq i}^{N} \sigma_i^2\sigma_j^2 \mathrm{tr}(M_{ij}M_{ji})$$

with $c_{m,i} = \sigma_i^4[\mathrm{tr}(M_{ii})\mathrm{tr}(M_{ii}) + \mathrm{tr}(M_{ii}^2) + \mathrm{tr}(M_{ii}M_{ii}')]$.

Since $\mathrm{E}(V'MV) = \sum_{i=1}^N \sigma_i^2 \mathrm{tr}(M_{ii})$, it entails

$$\begin{aligned}
\mathrm{Var}(V'MV) &= \mathcal{M}_1 + \mathcal{M}_2 + \mathcal{M}_3 + \mathcal{M}_4 - \Big(\sum_{i=1}^{N}\sigma_i^2 \mathrm{tr}(M_{ii})\Big)^2 \\
&= \sum_{i=1}^{N}\sum_{t=1}^{T}(\varrho_i - 3\sigma_i^4)m_{ii,tt}^2 + \sum_{i=1}^{N}\sum_{t=1}^{T}(a_{it} + 2e_{it} + 2f_{it}) \\
&\quad + \sum_{i=1}^{N}\sum_{j=1}^{N}\sigma_i^2\sigma_j^2\big(\mathrm{tr}(M_{ij}M_{ij}') + \mathrm{tr}(M_{ij}M_{ji})\big) \qquad \text{(C.1)} \\
&= \sum_{i=1}^{N}\sum_{t=1}^{T}(\varrho_i - 3\sigma_i^4)m_{ii,tt}^2 + \sum_{i=1}^{N}\sum_{t=1}^{T}(a_{it} + 2e_{it} + 2f_{it}) \\
&\quad + \mathrm{tr}(M\Sigma M'\Sigma) + \mathrm{tr}(M\Sigma M\Sigma) \\
&= O(NT),
\end{aligned}$$

where $\Sigma = \mathrm{diag}(\sigma_1^2, ..., \sigma_N^2) \otimes I_T$, and the last equation follows from Conditions 1–2.

Similarly, we can show

$$\begin{aligned}
\mathrm{Var}(b'V) &= \sum_{i=1}^{N}\sigma_i^2 b_i' b_i = O(NT), \\
\mathrm{E}(V'MVb'V) &= \sum_{i=1}^{N}\sum_{t=1}^{T}(\pi_i b_{i,t} m_{ii,tt} + g_{it}) = O(NT).
\end{aligned} \qquad \text{(C.2)}$$

As $\mathcal{LQ} = V'MV + b'V$, it follows that $\sigma_{\mathcal{LQ}}^2 = \mathrm{Var}(\mathcal{LQ}) = O(NT)$. By Theorem 14.4-1 in Bishop et al. (2007), that is $\mathcal{Y} - \mathrm{E}(\mathcal{Y}) = O_p(\sqrt{\mathrm{Var}(\mathcal{Y})})$ for a variable $\mathcal{Y}$, it yields the conclusion that $\mathcal{LQ} - \mu_{\mathcal{LQ}} = O_p(\sqrt{NT})$. □

**Proof for Theorem 3.2.** We focus on the proof based on the matrix assumption in Condition 3(ii) and the condition that both $N$ and $T$ go to infinity. Those proofs based on the conditional variance assumption in Condition 3(ii) or the small $N$ or $T$ case share similar arguments.

We suppose that $M$ is a symmetric matrix w.l.o.g., since $V'MV = V'\frac{M+M'}{2}V$ even if $M$ is asymmetric. Since $M_{ij} = M'_{ji}$, then the corresponding variance becomes

$$\begin{aligned}\sigma^2_{\mathcal{LQ}} = &\sum_{i=1}^{N}\sum_{t=1}^{T}(\varrho_i - 3\sigma_i^4)m^2_{ii,tt} + \sum_{i=1}^{N}\sum_{t=1}^{T}(a_{it} + 2e_{it} + 2f_{it} + 2g_{it} + 2\pi_i b_{i,t} m_{ii,tt}) \\ &+ 2\sum_{i=1}^{N}\sum_{j=1}^{N}\sigma_i^2\sigma_j^2 \mathrm{tr}(M_{ij}M'_{ij}) + \sum_{i=1}^{N}\sigma_i^2 b'_i b_i.\end{aligned} \tag{C.3}$$

Next, we rewrite

$$\mathcal{LQ} - \mu_{\mathcal{LQ}} = \sum_{i=1}^{N}\sum_{t=1}^{T}(q_{it} + q^\dagger_{it}),$$

where

$$q_{it} = 2\Big(\sum_{t^*=1}^{t-1} m_{ii,tt^*}v_{it^*}\Big)v_{it} + \Big(2\sum_{j=1}^{i-1}\sum_{t^*=1}^{T} m_{ij,tt^*}v_{jt^*} + b_{it}\Big)v_{it} \quad \text{and} \quad q^\dagger_{it} = m_{ii,tt}(v^2_{it} - \sigma^2_i). \tag{C.4}$$

Define the $\sigma$-field $\mathcal{F}_{it} = \mathcal{V}_{1T}\cup ... \cup\mathcal{V}_{i-1,T}\cup\mathcal{V}_{it}$ with $\mathcal{V}_{it} = \sigma(v_{it}, v_{i,t-1}, ...)$. Let $s = (i-1)T + t$. Then, we re-labeled $\mathcal{F}_{it}$ and $q_{it}$ into $\mathcal{F}_s$ and $q_s$ as follows:

$$\{\mathcal{F}_1, ..., \mathcal{F}_T, ..., \mathcal{F}_{(N-1)T+1}, ..., \mathcal{F}_{NT}\} := \{\mathcal{F}_{11}, ..., \mathcal{F}_{1T}, ..., \mathcal{F}_{N1}, ..., \mathcal{F}_{NT}\},$$

$$\{q_1, ..., q_T, ..., q_{(N-1)T+1}, ..., q_{NT}\} := \{q_{11}, ..., q_{1T}, ..., q_{N1}, ..., q_{NT}\}.$$

Since $\mathrm{E}(q_{it}|\mathcal{F}_{i,t-1}) = 0$ and $\mathrm{E}(q_{it}|\mathcal{F}_{i-1,T}) = 0$ by Condition 2, we know that $\mathrm{E}(q_s|\mathcal{F}_{s-1}) = 0$ (that is, $\{q_s, \mathcal{F}_s\}$ is a martingale difference sequence). Therefore, by the martingale difference CLT (see Theorem 3.2 in Hall and Heyde (1980)) for $\sum_{s=1}^{NT} q_s$ (also $\sum_{i=1}^{N}\sum_{t=1}^{T} q_{it}$), it suffices to prove the following three claims:

**Claim C.1.** $\sigma_{\mathcal{LQ}}^{-(2+\delta_1)}\sum_{i=1}^{N}\sum_{t=1}^{T}\mathrm{E}(|q_{it}|^{2+\delta_1}) = o(1)$ *for some* $\delta_1 > 0$.

**Claim C.2.** $\sigma_{\mathcal{LQ}}^{-2}\sum_{i=1}^{N}\sum_{t=1}^{T} q^2_{it} = 1 + o_p(1)$.

**Claim C.3.** $\sigma_{\mathcal{LQ}}^{-1}\sum_{i=1}^{N}\sum_{t=1}^{T} q^\dagger_{it} = o_p(1)$.

Note that for the proof with the conditional variance assumption in Condition 3(ii), Claim C.3 becomes unnecessary, since $q^\dagger_{it}$ in (C.4) can be included into $q_{it}$; in this case, similar conclusions as Claims C.1–C.2 can be proved in a straightforward manner. □

**Proof for Claim C.1.** Denote $r_1 = 2 + \delta_1$ for some $0 < \delta_1 < \delta/2$, and $r_2$ satisfying $r_1^{-1} + r_2^{-1} = 1$ and $0 < r_2 < 2$. Then, by (C.4) we have

$$|q_{it}| \leq \sum_{t^*=1}^{t-1} 2|m_{ii,tt^*}|^{\frac{1}{r_1}} |m_{ii,tt^*}|^{\frac{1}{r_2}} |v_{it^*}||v_{it}| + \sum_{j=1}^{i-1}\sum_{t^*=1}^{T} 2|m_{ij,tt^*}|^{\frac{1}{r_1}} |m_{ij,tt^*}|^{\frac{1}{r_2}} |v_{jt^*}||v_{it}| + |b_{it}||v_{it}|.$$

Next, by Hölder's inequality, it is not hard to see

$$\begin{aligned}|q_{it}| \leq &\Big(\sum_{t^*=1}^{t-1} 2^{r_1}|m_{ii,tt^*}||v_{it^*}|^{r_1}|v_{it}|^{r_1} + \sum_{j=1}^{i-1}\sum_{t^*=1}^{T} 2^{r_1}|m_{ij,tt^*}||v_{jt^*}|^{r_1}|v_{it}|^{r_1} + |v_{it}|^{r_1}\Big)^{\frac{1}{r_1}} \\ &\times \Big(\sum_{t^*=1}^{t-1}|m_{ii,tt^*}| + \sum_{j=1}^{i-1}\sum_{t^*=1}^{T}|m_{ij,tt^*}| + |b_{it}|^{r_2}\Big)^{\frac{1}{r_2}}.\end{aligned}$$

Note that $M$ is uniformly bounded in row and column, $\sup_{i,t} b_{it}^2 < \infty$, and $v_{it}$ is $L_{4+\delta}$-bounded with $4+\delta > 2r_1$. It implies that $\sup_{i,t} \mathrm{E}|q_{it}|^{r_1} = O(1)$. Since $\sigma_{\mathcal{LQ}}^{2+\delta_1} = O((NT)^{1+\frac{\delta_1}{2}})$ by Theorem 3.1, it follows that

$$\frac{1}{\sigma_{\mathcal{LQ}}^{2+\delta_1}} \sum_{i=1}^{N}\sum_{t=1}^{T} \mathrm{E}(|q_{it}|^{2+\delta_1}) = O\big((NT)^{-\frac{\delta_1}{2}}\big).$$

Hence, Claim C.1 holds. □

**Proof for Claim C.2.** By (C.4), we write

$$\frac{1}{NT}\sum_{i=1}^{N}\sum_{t=1}^{T} q_{it}^2 = \mathcal{B}_1 + \mathcal{B}_2 + \mathcal{B}_3, \tag{C.5}$$

where

$$\begin{aligned}\mathcal{B}_1 &= \frac{1}{NT}\sum_{i=1}^{N}\sum_{t=1}^{T} 4\big(\sum_{t^*=1}^{t-1} m_{ii,tt^*}v_{it^*}\big)^2 v_{it}^2 + \frac{1}{NT}\sum_{i=1}^{N}\sum_{t=1}^{T} 4b_{it}\big(\sum_{t^*=1}^{t-1} m_{ii,tt^*}v_{it^*}\big)v_{it}^2, \\ \mathcal{B}_2 &= \frac{1}{NT}\sum_{i=1}^{N}\sum_{t=1}^{T} \big(2\sum_{j=1}^{i-1}\sum_{t^*=1}^{T} m_{ij,tt^*}v_{jt^*} + b_{it}\big)^2 v_{it}^2, \\ \mathcal{B}_3 &= \frac{1}{NT}\sum_{i=1}^{N}\sum_{t=1}^{T} 8\big(\sum_{j=1}^{i-1}\sum_{t^*=1}^{T} m_{ij,tt^*}v_{jt^*}\big)\big((\sum_{t^*=1}^{t-1} m_{ii,tt^*}v_{it^*})v_{it}\big)v_{it}.\end{aligned}$$

For $\mathcal{B}_1$, we write its first item as

$$\frac{1}{NT}\sum_{i=1}^{N}\sum_{t=1}^{T} 4\big(\sum_{t^*=1}^{t-1} m_{ii,tt^*}v_{it^*}\big)^2 v_{it}^2 = \mathcal{B}_1^* + \mathcal{B}_1^{**},$$

where

$$\mathcal{B}_1^* = \frac{1}{NT}\sum_{i=1}^{N}\sum_{t=1}^{T} 4\Big(\sum_{t^*=t-\chi}^{t-1} m_{ii,tt^*} v_{it^*}\Big)^2 v_{it}^2.$$

To prove this item converges to its expectation, it suffices to show

$$\begin{aligned} &\text{(i)} \quad \mathcal{B}_1^* - \mathrm{E}(\mathcal{B}_1^*) = o_p(1), \quad \forall\, \chi \geq 1; \\ &\text{(ii)} \quad \mathrm{E}|\mathcal{B}_1^{**}| \to 0, \qquad \text{as } T, \chi \to \infty. \end{aligned} \tag{C.6}$$

For (i) in (C.6), it is given that

$$\mathcal{B}_1^* - \mathrm{E}(\mathcal{B}_1^*) = \frac{4}{NT}\sum_{i=1}^{N}\sum_{t=1}^{T}\sum_{c,c^*=1}^{\chi} g_{it,cc^*} = \sum_{c,c^*=1}^{\chi}\frac{4}{NT}\sum_{i=1}^{N}\sum_{t=1}^{T} g_{it,cc^*},$$

where

$$g_{it,cc^*} = m_{ii,t,t-c} m_{ii,t,t-c^*}[v_{it}^2 v_{i,t-c} v_{i,t-c^*} - \mathrm{E}(v_{it}^2 v_{i,t-c} v_{i,t-c^*})].$$

To prove (i), we only need to show that for each $i$,

$$\frac{1}{T}\sum_{t=1}^{T} g_{it,cc^*} = o_p(1).$$

Since $\{v_{it}\}$ is stationary and ergodic in $t$ with $\mathrm{E}(v_{it}^4) < \infty$, by Theorem 3.5.8 in Stout (1974) and Hölder's inequality, it follows that $\{v_{it}^2 v_{i,t-c} v_{i,t-c^*}\}$ is also stationary and ergodic in $t$ with $\mathrm{E}|v_{it}^2 v_{i,t-c} v_{i,t-c^*}| < \infty$. Hence, by using Lemma 10 in Dalla et al. (2014), we only need to show that $m_{it,cc^*}^* := m_{ii,t,t-c} m_{ii,t,t-c^*}$ satisfies

$$(a)\ \frac{1}{T}\sum_{t=1}^{T}|m_{it,cc^*}^*| = O(1); \qquad (b)\ \frac{1}{T}\sum_{t=2}^{T}|m_{it,cc^*}^* - m_{i,t-1,cc^*}^*| = o(1).$$

Note that (a) follows from the fact that $|m_{ii,t,t-c}| < \infty$ and $|m_{ii,t,t-c^*}| < \infty$, since $\sup_{i,t}\sum_{j=1}^{N}\sum_{t^*=1}^{T}|m_{ij,tt^*}| < \infty$ by Condition 1. For (b), it is obtained that

$$\begin{aligned} &T^{-1}\sum_{t=2}^{T}|m_{it,cc^*}^* - m_{i,t-1,cc^*}^*| \\ &= T^{-1}\sum_{t=2}^{T}|m_{ii,t,t-c} m_{ii,t,t-c^*} - m_{ii,t-1,t-1-c} m_{ii,t-1,t-1-c^*}| \\ &\leq T^{-1}\sum_{t=2}^{T}\big(|m_{ii,t,t-c} - m_{ii,t-1,t-1-c}||m_{ii,t,t-c^*}| + |m_{ii,t,t-c^*} - m_{ii,t-1,t-1-c^*}||m_{ii,t-1,t-1-c}|\big) \\ &< \infty, \end{aligned}$$

where the last inequality follows from Conditions 1 and 3. Hence, (i) in (C.6) holds.

To verify (ii) in (C.6), it is not hard to see

$$
\begin{aligned}
|\mathcal{B}_1^{**}| &= \Big|\frac{4}{NT}\sum_{i=1}^{N}\sum_{t=1}^{T} v_{it}^2\Big[\Big(\sum_{t^*=1}^{t-1} m_{ii,tt^*}v_{it^*}\Big)^2 - \Big(\sum_{t^*=t-\chi}^{t-1} m_{ii,tt^*}v_{it^*}\Big)^2\Big]\Big| \\
&= \Big|\frac{4}{NT}\sum_{i=1}^{N}\sum_{t=1}^{T} v_{it}^2\Big[\Big(\sum_{t^*=1}^{t-\chi-1} m_{ii,tt^*}v_{it^*}\Big)^2 + 2\Big(\sum_{t^*=1}^{t-\chi-1} m_{ii,tt^*}v_{it^*}\Big)\Big(\sum_{t^*=t-\chi}^{t-1} m_{ii,tt^*}v_{it^*}\Big)\Big]\Big| \\
&\le \frac{4}{NT}\sum_{i=1}^{N}\sum_{t=1}^{T} v_{it}^2\Big(\sum_{t^*=1}^{t-\chi-1} m_{ii,tt^*}v_{it^*}\Big)^2 + \Big[\frac{4}{NT}\sum_{i=1}^{N}\sum_{t=1}^{T} v_{it}^2\Big(\sum_{t^*=1}^{t-\chi-1} m_{ii,tt^*}v_{it^*}\Big)^2\Big]^{1/2} \\
&\quad \times \Big[\frac{4}{NT}\sum_{i=1}^{N}\sum_{t=1}^{T} v_{it}^2\Big(\sum_{t^*=t-\chi}^{t-1} m_{ii,tt^*}v_{it^*}\Big)^2\Big]^{1/2} \\
&:= \mathcal{B}_1^{***} + \sqrt{\mathcal{B}_1^{***}}\sqrt{\mathcal{B}_1^{*}},
\end{aligned}
$$

where the second equation is obtained by the fact $a^2 - b^2 = (a-b)^2 + 2(a-b)b$, and the inequality follows from Hölder's inequality. By Cauchy's inequality, it follows that

$$
\mathrm{E}|\mathcal{B}_1^{**}| \le \mathrm{E}(\mathcal{B}_1^{***}) + [\mathrm{E}(\mathcal{B}_1^{***})\mathrm{E}(\mathcal{B}_1^{*})]^{1/2}.
$$

Notably, $\mathrm{E}(\mathcal{B}_1^{*}) = O(1)$. Then, it remains to prove that $\mathrm{E}(\mathcal{B}_1^{***}) = o(1)$. As $T, \chi \to \infty$,

$$
\begin{aligned}
\mathrm{E}(\mathcal{B}_1^{***}) &= \frac{4}{NT}\sum_{i=1}^{N}\sum_{t=1}^{T} \mathrm{E}\Big[v_{it}^2\Big(\sum_{t^*=1}^{t-\chi-1} m_{ii,tt^*}v_{it^*}\Big)^2\Big] \\
&\le \frac{4}{NT}\sum_{i=1}^{N}\sum_{t=1}^{T} [\mathrm{E}(v_{it}^4)]^{1/2}\Big\{\mathrm{E}\Big[\Big(\sum_{t^*=1}^{t-\chi-1} m_{ii,tt^*}v_{it^*}\Big)^4\Big]\Big\}^{1/2} \\
&\le \frac{1}{NT}\sum_{i=1}^{N}\sum_{t=1}^{T}\sum_{t^*=1}^{t-\chi-1} m_{ii,tt^*}^2 \times O(1) = o(1),
\end{aligned}
$$

where the first inequality follows from Hölder's inequality, the second inequality is derived by Lemma 2.2 in Giraitis et al. (2017), and the last equality follows from Condition 3. Thus, (ii) in (C.6) holds. Back to (C.6), we have proven that the first item in $\mathcal{B}_1$ converges to its expectation. Similarly, we can show that the second item in $\mathcal{B}_1$ also converges to its expectation. Hence, we have $\mathcal{B}_1 - \mathrm{E}(\mathcal{B}_1) = o_p(1)$.

Now, we aim to prove that $\mathcal{B}_2 - \mathrm{E}(\mathcal{B}_2) = o_p(1)$. First, we have

$$
\frac{1}{NT}\sum_{i=1}^{N}\sum_{t=1}^{T}\Big\{\mathrm{E}\Big[\Big(2\sum_{j=1}^{i-1}\sum_{t^*=1}^{T} m_{ij,tt^*}v_{jt^*} + b_{it}\Big)^2 v_{it}^2|\mathcal{F}_{i-1,T}\Big] - \mathrm{E}\Big[\Big(2\sum_{j=1}^{i-1}\sum_{t^*=1}^{T} m_{ij,tt^*}v_{jt^*} + b_{it}\Big)^2 v_{it}^2\Big]\Big\}
$$

$$= \frac{1}{NT}\sum_{i=1}^{N}\sum_{t=1}^{T}\Big\{\Big(2\sum_{j=1}^{i-1}\sum_{t^*=1}^{T} m_{ij,tt^*}v_{jt^*}+b_{it}\Big)^2 - \mathrm{E}\Big[\Big(2\sum_{j=1}^{i-1}\sum_{t^*=1}^{T} m_{ij,tt^*}v_{jt^*}+b_{it}\Big)^2\Big]\Big\}\sigma_i^2$$

$$= O_p\Big(\frac{1}{\sqrt{NT}}\Big) = o_p(1), \tag{C.7}$$

where the first equation holds by Condition 2, and the second equation follows from Theorem 3.1 and the fact that

$$\begin{aligned}&\sum_{i=1}^{N}\sum_{t=1}^{T}\Big[\Big(\sum_{j=1}^{i-1}\sum_{t^*=1}^{T} m_{ij,tt^*}v_{jt^*}\Big)^2 + \Big(\sum_{j=1}^{i-1}\sum_{t^*=1}^{T} m_{ij,tt^*}v_{jt^*}\Big)b_{it}\Big]\sigma_i^2 \\ &= V'M^{-'}\Sigma_1 M^- V + b'\Sigma_1 M^- V.\end{aligned} \tag{C.8}$$

Here, $M^-$ is a uniformly bounded and lower triangular matrix and its $(i,j)$-th block $M^-_{ij} = M_{ij}$ when $i > j$, else $M^-_{ij} = 0$; and the matrix $\Sigma_1 := \mathrm{diag}(\sigma_1^2, ..., \sigma_N^2) \otimes I_T$ is also uniformly bounded.

By Theorem 3.1 and (C.8), it is not hard to see that $(NT)^{-1}\sum_{i=1}^{N}\sum_{t=1}^{T}(2\sum_{j=1}^{i-1}\sum_{t^*=1}^{T}$ $m_{ij,tt^*}v_{jt^*} + b_{it})^2 = O_p(1)$. Then, by Theorem 2.23 in Hall and Heyde (1980), we have

$$\frac{1}{NT}\sum_{i=1}^{N}\sum_{t=1}^{T}\Big\{\mathrm{E}\Big[\Big(2\sum_{j=1}^{i-1}\sum_{t^*=1}^{T} m_{ij,tt^*}v_{jt^*}+b_{it}\Big)^2 v_{it}^2|\mathcal{F}_{i-1,T}\Big] - \Big(2\sum_{j=1}^{i-1}\sum_{t^*=1}^{T} m_{ij,tt^*}v_{jt^*}+b_{it}\Big)^2 v_{it}^2\Big\}$$
$$= o_p(1).$$

Together with (C.7), it follows that $\mathcal{B}_2 - \mathrm{E}(\mathcal{B}_2) = o_p(1)$.

Note that $\mathcal{B}_3 - \mathrm{E}(\mathcal{B}_3) = o_p(1)$ by Hölder's inequality. Hence, according to (C.5), we have verified

$$\frac{1}{NT}\sum_{i=1}^{N}\sum_{t=1}^{T}[q_{it}^2 - \mathrm{E}(q_{it}^2)] = o_p(1).$$

Moreover, by (C.5) and some direct calculations, we can show

$$\begin{aligned}&\frac{1}{NT}\sum_{i=1}^{N}\sum_{t=1}^{T}\mathrm{E}(q_{it}^2) \\ &= \frac{1}{NT}\sigma^2_{\mathcal{LQ}} - \frac{1}{NT}\sum_{i=1}^{N}\sum_{t=1}^{T}(\varrho_i - 3\sigma_i^4)m^2_{ii,tt} - \frac{1}{NT}\sum_{i=1}^{N}\sum_{t=1}^{T} m_{ii,tt}\times\sum_{t^*=1,t^*\neq t}^{T}[m_{ii,t^*t^*}\varsigma_{i,t,t^*} \\ &\quad + \textstyle\sum_{t^\sharp=1,t^\sharp\neq t,t^*}^{T} m_{ii,t^*t^\sharp}\vartheta_{i,t,t^*,t^\sharp} + 2(m_{ii,tt^*}+m_{ii,t^*t})\varrho_{i,t,t^*} + 2b_{it^*}\pi_{i,t,t^*} + 2b_{i,t}\pi_i] \\ &= \frac{1}{NT}\sigma^2_{\mathcal{LQ}} + o(1),\end{aligned}$$

where $\sigma^2_{\mathcal{LQ}}$ is defined in (C.3), and the second equation follows from Hölder's inequality, Conditions 1–2, and the matrix assumption in Condition 3(ii). Therefore, it follows that Claim C.2 holds. □

**Proof for Claim C.3.** Under the matrix assumption in Condition 3(ii), we have

$$\frac{1}{NT}\mathrm{Var}\Big(\sum_{i=1}^{N}\sum_{t=1}^{T} q_{it}^{\dagger}\Big) = \frac{1}{NT}\sum_{i=1}^{N}\sum_{t=1}^{T} m_{ii,tt}^2 \varrho_i = o(1).$$

As $\sigma^2_{\mathcal{LQ}} = O(NT)$, it entails that Claim C.3 holds. □

## C.2 Proofs for the panel ARMA specification

To prove Theorems 4.1–4.3, we provide several lemmas below. Lemma C.1 is used for applying Theorem 3.1 to establish the asymptotics of $\hat{\lambda}$. Lemma C.2 is to investigate the initial values effect on the asymptotics of our estimators. Lemmas C.3–C.5 are necessary for the consistency of $\hat{\lambda}$. Lemmas C.6–C.7 are needed for the asymptotic normality of $\hat{\lambda}$.

**Lemma C.1.** *Under Assumption 4.1, we know that (i) $A_\phi$ and $B_\psi$ are non-stochastic and non-singular; (ii) $A_\phi$, $A_\phi^{-1}$, $\dot{A}_p$, $B_\psi$, $B_\psi^{-1}$, $\Sigma_\psi$, $\Sigma_\psi^{-1}$, $\dot{\Sigma}_q$, and $\ddot{\Sigma}_{qq^*}$ are uniformly bounded in row and column.*

**Lemma C.2.** *Let $M$ and $b$ be the matrices defined in Condition 1. Suppose that $M = I_N \otimes M_{11}$, where $M_{11}$ is a $T\times T$-dimensional matrix with $(t,t^*)$-th element $m_{11,tt^*}$, and $b = I_N \otimes b_1$ with $b_1$ being a $T\times 1$-dimensional vector with $t$-th element $b_{1t}$. Denote $\mathcal{LQ}^\dagger = \hat{U}_{\theta_{01}} M \hat{U}_{\theta_{01}} + b'\hat{U}_{\theta_{01}} - UMU - b'U$. Then, we have*

$$\mathrm{E}(\mathcal{LQ}^\dagger) = O(N) \quad \textit{and} \quad \mathcal{LQ}^\dagger - \mathrm{E}(\mathcal{LQ}^\dagger) = O_p(\sqrt{N}). \tag{C.9}$$

**Lemma C.3.** $(NT)^{-1}[\hat{Q}_\lambda - \mathrm{E}(Q_\lambda)] = o_p(1)$, *where $Q_\lambda$ is defined in the same way as $\hat{Q}_\lambda$ with $\hat{U}_{\theta_1}$ replaced by $U_{\theta_1}$.*

**Lemma C.4.** $(NT)^{-1}\hat{Q}_\lambda$ *is stochastically equicontinuous.*

**Lemma C.5.** $\hat{\lambda}$ *is uniquely and globally identified.*

**Lemma C.6.** $(1/\sqrt{NT})[D - \mathrm{E}(D)] \xrightarrow{d} N(0, \lim \Omega_1)$.

**Lemma C.7.** $D^\dagger - \mathrm{E}(D^\dagger) = O_p(\sqrt{N})$, $\mathrm{E}(D) = O(N)$, *and* $\mathrm{E}(D^\dagger) = O(N)$.

**Proof for Lemma C.1.** First, part (i) follows from the fact that $A_\phi$ and $B_\psi$ are lower triangular matrices with diagonal elements 1. Second, it is straightforward to show the uniform boundedness properties of $A_\phi$ and $\dot{A}_p$. By Lemma 2.1 in Bühlmann (1995), we know that if Assumption 4.1(ii) holds, the functions $\phi^*(z)^{-1} = \sum_{i=0}^{\infty} \phi_i^* z^i$ and $\psi^*(z)^{-1} = \sum_{i=0}^{\infty} \psi_i^* z^i$ have the properties $\sum_{i=1}^{\infty} |\phi_i^*| < \infty$ and $\sum_{i=1}^{\infty} |\psi_i^*| < \infty$. It follows that $A_\phi^{-1}$ is uniformly bounded in row and column. Similarly, $B_\psi$, $B_\psi^{-1}$, and $\dot{B}_q = \partial B_\psi / \partial \psi_q$ are uniformly bounded in row and column. In view of $\Sigma_\psi = B_\psi B_\psi'$ and the sub-multiplicative property of the matrix norm, we know that $\Sigma_\psi$, $\Sigma_\psi^{-1}$, $\dot{\Sigma}_q$, and $\ddot{\Sigma}_{qq^*}$ are also uniformly bounded in row and column. Hence, part (ii) holds. □

**Proof for Lemma C.2.** We first consider the panel ARMA$(1,1)$ specification. In this case,

$$\hat{u}_{it,\theta_{01}} = y_{it} - \mu_{0i} - x_{it}\beta_0 - \phi_0 y_{i,t-1} - \psi_0 \hat{u}_{i,t-1,\theta_{01}},$$
$$u_{it} = y_{it} - \mu_{0i} - x_{it}\beta_0 - \phi_0 y_{i,t-1} - \psi_0 u_{i,t-1},$$

where the initial values $y_{i0} = \hat{u}_{i0,\theta_{01}} = 0$ are used for the computation of $\hat{u}_{it,\theta_{01}}$. Hence,

$$\Delta_{1,it} := \hat{u}_{it,\theta_{01}} - u_{it} = (-\psi_0)^{t-1}(\phi_0 y_{i0} + \psi_0 u_{i0}) \tag{C.10}$$

for each $i$ and $t$. Next, we can obtain

$$\hat{u}_{i,\theta_{01}} M_{11} \hat{u}_{i,\theta_{01}} + b_1' \hat{u}_{i,\theta_{01}} - u_i M_{11} u_i - b_1' u_i = \mathcal{M}_{i,1} + \mathcal{M}_{i,2} + \mathcal{M}_{i,3} + \mathcal{M}_{i,4}$$

for each $i$, where

$$\mathcal{M}_{i,1} = \sum_{t=1}^{T}\sum_{t^*=1}^{T} m_{11,tt^*}\Delta_{1,it}u_{it^*}, \qquad \mathcal{M}_{i,2} = \sum_{t=1}^{T}\sum_{t^*=1}^{T} m_{11,tt^*}u_{it}\Delta_{1,it^*},$$
$$\mathcal{M}_{i,3} = \sum_{t=1}^{T}\sum_{t^*=1}^{T} m_{11,tt^*}\Delta_{1,it}\Delta_{1,it^*}, \quad \mathcal{M}_{i,4} = \sum_{t=1}^{T} b_{it}\Delta_{1,it}.$$

As $\mathcal{L}\mathcal{Q}^\dagger = \sum_{i=1}^{N}(\mathcal{M}_{i,1} + \mathcal{M}_{i,2} + \mathcal{M}_{i,3} + \mathcal{M}_{i,4})$ and $u_{it}$ is independent across $i$ and uncorrelated over $t$, we have

$$\mathrm{E}(\mathcal{L}\mathcal{Q}^\dagger) = \sum_{i=1}^{N}\mathrm{E}(\mathcal{M}_{i,3}) + \sum_{i=1}^{N}\mathrm{E}(\mathcal{M}_{i,4})$$

$$= \sum_{i=1}^{N}\sum_{t=1}^{T}\sum_{t^*=1}^{T} m_{11,tt^*}(-\psi_0)^{t+t^*-2}\mathrm{E}(\phi_0 y_{i0}+\psi_0 u_{i0})^2 + \sum_{i=1}^{N}\sum_{t=1}^{T}(-\psi_0)^{t-1}\mathrm{E}[b_{1t}(\phi_0 y_{i0}+\psi_0 u_{i0})]$$
$$= O(N), \tag{C.11}$$

where the last equation follows from the $L_{4+\delta}$-boundedness of $y_{it}$ and $u_{it}$, the uniform boundedness of $M_{11}$, and the condition of $|\psi_0| < 1$ by Assumption 4.1.

Similarly, we can show

$$\mathrm{Var}(\mathcal{M}_{i,1}) = \mathrm{E}\Big(\sum_{t=1}^{T}\sum_{t^*=1}^{T} m_{11,tt^*}\Delta_{1,it}u_{it^*}\Big)^2$$
$$= \sum_{t=1}^{T} m_{11,tt}\mathrm{E}(\Delta_{1,it}^2 u_{it}^2) + \sum_{t=1}^{T}\sum_{t^*=1,t^*\neq t}^{T}\big[2m_{11,tt^*}m_{11,t^*t^*}\mathrm{E}(\Delta_{1,it}\Delta_{1,it^*}u_{it^*}^2) + m_{11,tt^*}^2\mathrm{E}(\Delta_{1,it}^2 u_{it^*}^2)\big]$$
$$= O(1),$$

and further prove

$$\mathrm{Var}(\mathcal{LQ}^\dagger) = \sum_{i=1}^{N}\mathrm{Var}(\mathcal{M}_{i,1}+\mathcal{M}_{i,2}+\mathcal{M}_{i,3}+\mathcal{M}_{i,4}) = O(N). \tag{C.12}$$

As $\mathcal{Y} - \mathrm{E}(\mathcal{Y}) = O_p(\sqrt{\mathrm{Var}(\mathcal{Y})})$ for a variable $\mathcal{Y}$, it yields that (C.9) holds for the panel ARMA$(1,1)$ specification.

For the general panel ARMA$(P,Q)$ specification, we suppose that $P = Q$ w.l.o.g. Similar to (C.10), it is obtained that

$$\text{when } t \le P, \quad \Delta_{1,it} = \sum_{p=t}^{P}\phi_p y_{i,t-p} + \sum_{q=1}^{t-1}\psi_q\Delta_{1,iq} + \sum_{q^*=t}^{Q}\psi_{q^*}u_{i,t-q^*};$$
$$\text{when } t > P, \quad \Delta_{1,it} = \sum_{q=1}^{Q}\psi_q\Delta_{1,iq}.$$

Like (C.11)–(C.12), we have

$$\mathrm{E}(\mathcal{LQ}^\dagger) = \sum_{t=1}^{T}\sum_{t^*=1}^{T} m_{11,tt^*}\mathrm{E}(\Delta_{1,it}\Delta_{1,it^*}) + \sum_{t=1}^{T}\mathrm{E}(b_{1t}\Delta_{1,it}) = O(N) \tag{C.13}$$

and $\mathrm{Var}(\mathcal{LQ}^\dagger) = O(N)$. Then, $\mathcal{LQ}^\dagger - \mathrm{E}(\mathcal{LQ}^\dagger) = O_p(\sqrt{N})$. □

**Proof for Lemma C.3.** By (2.2)–(2.3), we have

$$V_{\phi,\beta} = (I_N \otimes A_\phi A^{-1}B)\hat{U}_{\theta_{01}} + (I_N \otimes A_\phi A^{-1})R - X\beta,$$

where $R = X\beta_0 + (I_N \otimes l_T)\mu_0$. Then,

$$\hat{Q}_\lambda = V'_{\phi,\beta}(I_N \otimes (\Sigma_\psi^{-1} - C_\psi))V_{\phi,\beta} = \hat{\mathcal{I}}_1 + \hat{\mathcal{I}}_2 + \hat{\mathcal{I}}_3 \tag{C.14}$$

with

$$\hat{\mathcal{I}}_1 = \hat{U}'_{\theta_{01}}(I_N \otimes B'A^{-1\prime}A'_\phi(\Sigma_\psi^{-1} - C_\psi)A_\phi A^{-1}B)\hat{U}_{\theta_{01}},$$
$$\hat{\mathcal{I}}_2 = \hat{U}'_{\theta_{01}}(I_N \otimes B'A^{-1\prime}A'_\phi(\Sigma_\psi^{-1} - C_\psi))\big((I_N \otimes A_\phi A^{-1})R - X\beta\big),$$
$$\hat{\mathcal{I}}_3 = \big((I_N \otimes A_\phi A^{-1})R - X\beta\big)'(I_N \otimes (\Sigma_\psi^{-1} - C_\psi))\big((I_N \otimes A_\phi A^{-1})R - X\beta\big).$$

Likewise, $\mathcal{I}_i$ with $i = 1, 2$ are defined with $\hat{U}_{\theta_{01}}$ replaced by $U$, and $\mathcal{I}_3 = \hat{\mathcal{I}}_3$. Then, $Q_\lambda = \mathcal{I}_1 + \mathcal{I}_2 + \mathcal{I}_3$. By Lemma C.1 and the sub-multiplicative property of the matrix norm, it follows that $I_N \otimes B'A^{-1\prime}A'_\phi(\Sigma_\psi^{-1} - C_\psi)A_\phi A^{-1}B$ and other matrices in $\hat{\mathcal{I}}_i$ are uniformly bounded in row and column. Hence, by Lemma C.2, we can show that $(NT)^{-1}(\hat{\mathcal{I}}_i - \mathcal{I}_i) = o_p(1)$. Moreover, by Theorem 3.1, we have $(NT)^{-1}[\mathcal{I}_i - \mathrm{E}(\mathcal{I}_i)] = o_p(1)$. Hence, by (C.14), it entails that $(NT)^{-1}[\hat{Q}_\lambda - \mathrm{E}(Q_\lambda)] = o_p(1)$. □

**Proof for Lemma C.4.** It suffices to show the $L_1$-boundedness of $(NT)^{-1}\partial\hat{Q}_\lambda/\partial\lambda$. Using the same idea as for Lemma C.3, we can prove

$$\frac{1}{NT}\Big\|\frac{\partial \hat{Q}_\lambda}{\partial \beta}\Big\| \le \frac{1}{NT}\big\|V'_{\phi,\beta}(I_N \otimes \Sigma_\psi^{-1})X\big\| + \frac{1}{NT}\big\|V'_{\phi,\beta}(I_N \otimes C_\psi)X\big\| = O(1), \tag{C.15}$$

where the last equation follows by Assumption 4.2, Lemmas C.1–C.2, and Theorem 3.1. Similarly, we can have $(NT)^{-1}\|\partial\hat{Q}_\lambda/\partial\lambda\| = O(1)$. □

**Proof for Lemma C.5.** By Lemma C.2, it suffices to prove that $\lim(NT)^{-1}\mathrm{E}(Q_\lambda)$ reaches its unique minimum at $\lambda = \lambda_0$. For $\mathcal{I}_i$ in $Q_\lambda$, since $\mathrm{E}(\mathcal{I}_2) = 0$, we only need to show

$$(i) \lim \frac{1}{NT}\mathrm{E}(\mathcal{I}_1) \ge \lim \frac{1}{NT}\mathrm{E}(\mathcal{I}_{01}) \quad \text{and} \quad (ii) \lim \frac{1}{NT}\mathrm{E}(\mathcal{I}_3) \ge \lim \frac{1}{NT}\mathrm{E}(\mathcal{I}_{03}), \tag{C.16}$$

where the equality is reached if and only if $\lambda = \lambda_0$.

For (i), since $C_\psi = (l'_T\Sigma_\psi^{-1}l_T)^{-1}\Sigma_\psi^{-1}l_T l'_T\Sigma_\psi^{-1}$, by Lemma C.1 we have $\mathrm{tr}(B'A^{-1\prime}A'_\phi C_\psi A_\phi A^{-1}B) = O(1)$. Then,

$$\lim \frac{1}{NT}\mathrm{E}(\mathcal{I}_1) = \lim \frac{1}{NT}\sum_{i=1}^{N}\mathrm{E}[u'_{i,\theta_{01}}B'A^{-1\prime}A'_\phi\Sigma_\psi^{-1}A_\phi A^{-1}Bu_{i,\theta_{01}}]. \tag{C.17}$$

Notably, $\sum_{i=1}^{N} u'_{i,\theta_{01}} B'A^{-1'}A'_{\phi}\Sigma_{\psi}^{-1}A_{\phi}A^{-1}Bu_{i,\theta_{01}}$ is sum of $N$ different objective functions, each of which is the objective function for the LS estimation of the univariate ARMA model. Following the proof for estimation identification in Ling (2007), we can show that the RHS of (C.17) reaches its unique minimum at $\lambda = \lambda_0$, and the minimum value equals to $\lim(NT)^{-1}\mathrm{E}(\mathcal{I}_{01})$. Hence, (i) in (C.16) holds.

For (ii), note that $\mathcal{I}_3 = M_3'M_3$ with $M_3 = (I_N \otimes (I_T - (l_T'\Sigma_{\psi}^{-1}l_T)^{-1}\Sigma_{\psi}^{-1/2}l_T l_T'\Sigma_{\psi}^{-1}))\big((I_N \otimes A_{\phi}A^{-1})R - X\beta\big)$. Then, $\mathrm{E}(\mathcal{I}_3)$ reaches its minimum value zero, if and only if $M_3 = 0$. Furthermore, we know that $M_3 = 0$ holds if and only if $\lambda = \lambda_0$, since $X$ is not almost surely equal to zero under Assumption 4.1. Then, we obtain (ii) in (C.16). □

**Proof for Lemma C.6.** From (B.1), we know that all terms in $D$ have the linear-quadratic form in $U$ with some uniformly bounded weight matrices. Then, we can check that all of those matrices satisfy the matrix assumptions (a)–(c) in Condition 3(ii). For example, the involving matrix $M^{\star} := B_{\psi}'H_qB_{\psi}$ can be divided into two parts as follows:

$$M^{\star} = -B_{\psi}'\Sigma_{\psi}^{-1}\dot{\Sigma}_q\Sigma_{\psi}^{-1}B_{\psi} + B_{\psi}'[2\Sigma_{\psi}^{-1}\dot{\Sigma}_qC_{\psi} - \mathrm{tr}(\dot{\Sigma}_qC_{\psi})C_{\psi}]B_{\psi}. \tag{C.18}$$

The diagonals of the first part of the RHS of (C.18) are zero, and those of the second part are $O(T^{-1})$ as $C_{\psi} = (l_T'\Sigma_{\psi}^{-1}l_T)^{-1}\Sigma_{\psi}^{-1}l_Tl_T'\Sigma_{\psi}^{-1}$. Then, $M^{\star}$ satisfies the asymptotically vanishing diagonal assumption (a). Next, denote the $(i,j)$-th block matrix of $M^{\star}$ as $M_{ij}^{\star} = [m_{ij,tt^*}^{\star}]$. Clearly, $m_{ii,t,t-t^*}^{\star} - m_{ii,t-t^*-1}^{\star} = o(1)$ for any $1 \le t^* < T-1$, implying that assumption (b) holds for $M^{\star}$. Moreover, by Assumption 4.1 and (C.18), it is easy to obtain that $m_{ii,tt^*}^{\star} = O(c^{t-t^*}) + O(T^{-1})$ with $|c| < 1$. Hence, assumption (c) holds for $M^{\star}$. For other matrices within $D$, they can be analyzed similarly. Now, by Theorem 3.2, the desirable result holds. □

**Proof for Lemma C.7.** By Lemma C.1, the sub-multiplicative property of the matrix norm, and the fact that $\mathrm{tr}(C) = O(1)$, we can show that all of $\mathrm{tr}(B'C\dot{A}_pA^{-1}B)$, $\mathrm{tr}(B'\Sigma^{-1}\dot{\Sigma}_qCB)$, and $\mathrm{tr}(B'CB)$ are $O(1)$. Hence, since $\mathrm{tr}(A \otimes B) = \mathrm{tr}(A)\mathrm{tr}(B)$ for any two matrices $A$ and $B$, it follows that $\mathrm{E}(D)$ in (B.2) is $O(N)$.

By Lemma C.1 and (B.1), we can see that $D^{\dagger}$ has the structure as in $\mathcal{LQ}^{\dagger}$. Then, by Lemma C.2, we have $\mathrm{E}(D^{\dagger}) = O(N)$ and $D^{\dagger} - \mathrm{E}(D^{\dagger}) = O_p(\sqrt{N})$. □

Now, we are ready to provide the proof for Theorem 4.1.

**Proof for Theorem 4.1.** By Theorem 4.1.1 in Amemiya (1985), the consistency of $\hat{\lambda}$ follows from Lemmas C.3–C.5.

For the asymptotic normality, by Taylor's expansion we have

$$\sqrt{NT}(\hat{\lambda}-\lambda_0)=\frac{1}{\sqrt{NT}}\Gamma_1^{*-1}\big\{[D-\mathrm{E}(D)]+[D^{\dagger}-\mathrm{E}(D^{\dagger})]+\mathrm{E}(D)+\mathrm{E}(D^{\dagger})\big\},\tag{C.19}$$

where $\Gamma_1^*$ is a $(D_x+P+Q)\times(D_x+P+Q)$ matrix with $(i,j)$-th entry $\gamma_{1,ij}=-(NT)^{-1}$ $\partial^2\hat{Q}_{\lambda^*_{ij}}/\partial\lambda_i\partial\lambda_j$, and $\lambda^*_{ij}\in\Theta_\lambda$ lies between $\hat{\lambda}$ and $\lambda_0$.

For $\Gamma_1^{*-1}$, we need to show

$$\Gamma_1^{*-1}=\Gamma_1^{-1}+O_p\Big(\max\Big(\frac{1}{\sqrt{NT}},\frac{1}{T}\Big)\Big).\tag{C.20}$$

Recall that $\hat{S}=\partial^2\hat{Q}_\lambda/\partial\lambda\partial\lambda'\big|_{\lambda=\lambda_0}$. Similar to Lemmas C.6–C.7, we have

$$\begin{aligned}\frac{1}{NT}\hat{S}&=\frac{1}{NT}[S-\mathrm{E}(S)]+\frac{1}{NT}[S^{\dagger}-\mathrm{E}(S^{\dagger})]+\frac{1}{NT}\mathrm{E}(S)+\frac{1}{NT}\mathrm{E}(S^{\dagger})\\&=O_p\Big(\frac{1}{\sqrt{NT}}\Big)+O_p\Big(\frac{1}{\sqrt{NT^2}}\Big)-\Gamma_1+O\Big(\frac{1}{T}\Big).\end{aligned}$$

Then,

$$\begin{aligned}\Gamma_1^*&=\Big(\Gamma_1^*+\frac{1}{NT}\hat{S}\Big)-\Big(\frac{1}{NT}\hat{S}+\Gamma_1\Big)+\Gamma_1\\&=\sup_{i,j}|\lambda^*_{ij}-\lambda_0|O_p(1)+O_p\Big(\max\Big(\frac{1}{\sqrt{NT}},\frac{1}{T}\Big)\Big)+\Gamma_1,\end{aligned}\tag{C.21}$$

where $|\lambda^*_{ij}-\lambda_0|$ is the Euclidean norm of $\lambda^*_{ij}-\lambda_0$, and the term of $O_p(1)$ follows from the fact that $(NT)^{-1}\|\partial^3\hat{Q}_\lambda/\partial\lambda_i\partial\lambda_j\partial\lambda_k\|=O(1)$ for all $i$, $j$, and $k$ implied via similar arguments as for (C.15). Since $\hat{\lambda}-\lambda_0=o_p(1)$ and $\lambda^*_{ij}$ lies between $\hat{\lambda}$ and $\lambda_0$, it implies that $\sup_{i,j}|\lambda^*_{ij}-\lambda_0|=o_p(1)$. By Assumption 4.4 and (C.21), we have $\Gamma_1^{*-1}=O_p(1)$. Together with Lemmas C.6–C.7 and (C.19), it yields

$$\hat{\lambda}-\lambda_0=\frac{1}{\sqrt{NT}}\Big(O_p(1)\Big(O_p(1)+O\Big(\sqrt{\frac{N}{T}}\Big)\Big)\Big)=O_p\Big(\max\Big(\frac{1}{\sqrt{NT}},\frac{1}{T}\Big)\Big).\tag{C.22}$$

Back to (C.21), it follows that (C.20) holds.

Finally, by (C.19)–(C.20) we have

$$\sqrt{NT}(\hat{\lambda}-\lambda_0)=\frac{1}{\sqrt{NT}}\Gamma_1^{-1}[D-\mathrm{E}(D)]+\frac{1}{\sqrt{NT}}\Gamma_1^{-1}[\mathrm{E}(D)+\mathrm{E}(D^{\dagger})]$$

$$+ O_p\Big( \max\Big(\frac{1}{T}, \sqrt{\frac{N}{T^3}}\Big)\Big), \tag{C.23}$$

which yields the result by Lemmas C.6–C.7. □

**Proof for Theorem 4.2.** For $\hat{\mu}_{\hat{\lambda},i}$, we can show

$$\begin{aligned}
\hat{\mu}_{\hat{\lambda},i} - \mu_{0i} &= (l_T'\Sigma_{\hat{\psi}}^{-1}l_T)^{-1}l_T'\Sigma_{\hat{\psi}}^{-1}(A_{\hat{\phi}}y_i - x_i'\hat{\beta}) - \mu_{0i} \\
&= (l_T'\Sigma^{-1}l_T)^{-1}l_T'\Sigma^{-1}(Ay_i - x_i'\beta_0) - \mu_{0i} + O_p\Big( \max\Big(\frac{1}{\sqrt{NT}}, \frac{1}{T}\Big)\Big) \\
&= (l_T'\Sigma^{-1}l_T)^{-1}l_T'B^{-1\prime}\hat{u}_{i,\theta_{01}} + O_p\Big( \max\Big(\frac{1}{\sqrt{NT}}, \frac{1}{T}\Big)\Big) \\
&= (l_T'\Sigma^{-1}l_T)^{-1}l_T'B^{-1\prime}u_i + O_p\Big( \max\Big(\frac{1}{\sqrt{NT}}, \frac{1}{T}\Big)\Big),
\end{aligned}$$

where the four equations hold by (2.4), (C.22), (2.2), and Lemma C.2, respectively. Then, the conclusion follows directly. □

**Proof for Theorem 4.3.** First, we consider the asymptotic result for $\hat{\lambda}_A$. By Theorem 4.1 and (4.3), it suffices to show

$$(i)\ \sqrt{\frac{N}{T}}(\hat{c}_1 - c_1) = o_p(1); \qquad (ii)\ \sqrt{\frac{N}{T}}(\hat{c}_1^\dagger - c_1^\dagger) = o_p(1). \tag{C.24}$$

For (i) in (C.24), we denote $\Delta_1 := \mathrm{E}(D)$. Let $\hat{\Delta}_1$ and $\hat{\Gamma}_1$ be the plug-in estimators of $\Delta_1$ and $\Gamma_1$, respectively. Like (C.20), we can show

$$\frac{1}{N}\hat{\Delta}_1 - \frac{1}{N}\Delta_1 = O_p\Big( \max\Big(\frac{1}{\sqrt{NT}}, \frac{1}{T}\Big)\Big) \text{ and } \hat{\Gamma}_1 - \Gamma_1 = O_p\Big( \max\Big(\frac{1}{\sqrt{NT}}, \frac{1}{T}\Big)\Big).$$

Then,

$$\sqrt{\frac{N}{T}}(\hat{c}_1 - c_1) = \sqrt{\frac{N}{T}}\Big[(\hat{\Gamma}_1^{-1} - \Gamma_1^{-1})\frac{1}{N}\hat{\Delta}_1 + \Gamma_1^{-1}\Big(\frac{1}{N}\hat{\Delta}_1 - \frac{1}{N}\Delta_1\Big)\Big] = O_p\Big( \max\Big(\frac{1}{T}, \sqrt{\frac{N}{T^3}}\Big)\Big).$$

For (ii) in (C.24), it can be proved via similar arguments.

Next, we prove the asymptotic result for $\hat{\lambda}_J$. By Theorems 3.2 and 4.1, we have

$$\sqrt{NT}(\hat{\lambda} - \lambda_0) = \frac{1}{\sqrt{NT}}\sum_{i=1}^{N}\sum_{t=1}^{T}(\mathcal{D}_{it} + \mathcal{C}_{it}) + o_p(1),$$

where $\{\mathcal{D}_{it}\}$, as a martingale difference process over $t$ with mean zero, determines the asymptotic variance of $\hat{\lambda}$, and $\{\mathcal{C}_{it}\}$ determines the asymptotics bias of $\hat{\lambda}$. Then, the

asymptotic distribution of $\hat{\lambda}$ is derived in Theorem 4.1, and that of $\hat{\lambda}_1$ (or $\hat{\lambda}_2$) can be obtained similarly based on observations $t \in \{1, 2, ..., \lfloor T/2 \rfloor\}$ (or $t \in \{\lfloor T/2 \rfloor + 1, ..., T\}$). Denote the vector $\hat{\boldsymbol{\lambda}} = (\hat{\lambda}', \hat{\lambda}_1', \hat{\lambda}_2')'$. Then, it is straightforward to show

$$\sqrt{NT}\left(\hat{\boldsymbol{\lambda}} - \begin{bmatrix}1\\1\\1\end{bmatrix} \otimes \lambda_0 - \begin{bmatrix}1\\2\\2\end{bmatrix} \otimes \frac{1}{T}(c_1 + c_1^{\dagger})\right) \xrightarrow{\mathrm{d}} N\left(0, \begin{bmatrix}1 & 1 & 1\\1 & 2 & 0\\1 & 0 & 2\end{bmatrix} \otimes \Sigma_1\right).$$

Since $\hat{\lambda}_J = (2, -1/2, -1/2)\hat{\boldsymbol{\lambda}}$, the asymptotic distribution of $\hat{\lambda}_J$ follows directly. □

## C.3 Proofs for the panel GARCH specification

In Section 4.3, $\hat{G}$, $\check{G}$, $\tilde{G}$, $\bar{G}$, and $G$ with their differences are defined for analyzing the initial values effect, the estimation effects of $\lambda_0$, $\mu_0$, and $\omega_0$. Similarly, for the objective function $\hat{L}_{\zeta,\hat{\omega}}$, we define $\check{L}_{\zeta,\check{\omega}}$, $\tilde{L}_{\zeta,\tilde{\omega}}$, $\bar{L}_{\zeta,\bar{\omega}}$, and $L_{\zeta,\omega_0}$ with their differences $L_{\zeta}^{\dagger} = \hat{L}_{\zeta,\hat{\omega}} - \check{L}_{\zeta,\check{\omega}}$, $L_{\zeta}^{\S} = \check{L}_{\zeta,\check{\omega}} - \tilde{L}_{\zeta,\tilde{\omega}}$, $L_{\zeta}^{\sharp} = \tilde{L}_{\zeta,\tilde{\omega}} - \bar{L}_{\zeta,\bar{\omega}}$, and $L_{\zeta}^{\flat} = \bar{L}_{\zeta,\bar{\omega}} - L_{\zeta,\omega_0}$.

For the consistency and asymptotic normality of $\hat{\zeta}$, Lemmas C.8 and C.9 below are needed, respectively.

**Lemma C.8.**

$$\textit{(i)}\ \frac{1}{NT}L_{\zeta}^{\dagger} = o_p(1); \quad \textit{(ii)}\ \frac{1}{NT}L_{\zeta}^{\S} = o_p(1); \quad \textit{(iii)}\ \frac{1}{NT}L_{\zeta}^{\sharp} = o_p(1); \quad \textit{(iv)}\ \frac{1}{NT}L_{\zeta}^{\flat} = o_p(1).$$

**Lemma C.9.**

$$\textit{(i)}\ \frac{1}{\sqrt{NT}}G^{\dagger} = \frac{1}{\sqrt{NT}}\Delta^{\dagger} + o_p(1);$$

$$\textit{(ii)}\ \frac{1}{\sqrt{NT}}G^{\S} = \frac{1}{\sqrt{NT}}\Pi\Gamma_1^{-1}(D - \mathrm{E}(D)) + \frac{1}{\sqrt{NT}}\Delta^{\S} + o_p(1);$$

$$\textit{(iii)}\ \frac{1}{\sqrt{NT}}G^{\sharp} = \frac{1}{2\sqrt{NT}}\sum_{i=1}^{N}\sum_{t=1}^{T}\mathrm{E}(\mathcal{O}_{23,it}^{\sharp})u_{it} + \frac{1}{\sqrt{NT}}\Delta^{\sharp} + o_p(1);$$

$$\textit{(iv)}\ \frac{1}{\sqrt{NT}}G^{\flat} = -\frac{1}{2\sqrt{NT}}\sum_{i=1}^{N}\sum_{t=1}^{T}\mathrm{E}\Big(\frac{1}{h_{it}^2}\frac{\partial h_{it}}{\partial \zeta}\Big)(u_{it}^2 - h_{it}) + \frac{1}{\sqrt{NT}}\Delta^{\flat} + o_p(1),$$

*where $\mathcal{O}_{23,it}^{\sharp}$, $\Delta^{\dagger}$, $\Delta^{\S}$, $\Delta^{\sharp}$, and $\Delta^{\flat}$ are defined in (B.10), (C.40), (C.46), (C.55), and (C.62), respectively.*

We give the proof of Lemma C.8 for the ARMA(1,1)–GARCH(1,1) model below:

$$\begin{aligned} y_{it} &= \mu_{0i} + x_{it}'\beta_0 + \phi_0 y_{i,t-1} + \psi_0 u_{i,t-1} + u_{it}, \\ u_{it} &= \sqrt{h_{it}}\epsilon_{it} \text{ with } h_{it} = (1 - \tau_0 - \nu_0)\omega_{0i} + \tau_0 u_{i,t-1}^2 + \nu_0 h_{i,t-1}. \end{aligned} \tag{C.25}$$

For the general ARMA$(P,Q)$–GARCH$(L,K)$ model, the proof is similar and thus not provided for ease of presentation.

**Proof for Lemma C.8(i).** Note that

$$\begin{aligned}\hat{u}_{it} &= y_{it} - \hat{\mu}_{i,\hat{\lambda}} - x_{it}'\hat{\beta} - \hat{\phi} y_{i,t-1} - \hat{\psi}\hat{u}_{i,t-1},\\ \check{u}_{it} &= y_{it} - \tilde{\mu}_{i,\hat{\lambda}} - x_{it}'\hat{\beta} - \hat{\phi} y_{i,t-1} - \hat{\psi}\check{u}_{i,t-1},\end{aligned} \tag{C.26}$$

where the initial values $y_{i0} = \hat{u}_{i0} = 0$ are used for the computation of $\hat{u}_{it}$, and

$$\begin{aligned}\hat{\mu}_{i,\hat{\lambda}} &= (l_T'\Sigma_{\hat{\psi}}^{-1} l_T)^{-1} l_T' B_{\hat{\psi}}'^{-1} B_{\hat{\psi}}^{-1}(A_{\hat{\phi}} y_i - x_i\hat{\beta}),\\ \tilde{\mu}_{i,\hat{\lambda}} &= (1+\hat{\psi})\frac{1}{T}\sum_{t=1}^{T}(1+\hat{\psi}\mathcal{B})^{-1}(y_{it} - x_{it}'\hat{\beta} - \hat{\phi} y_{i,t-1}).\end{aligned} \tag{C.27}$$

First, we study the differences $\hat{\mu}_{i,\hat{\lambda}} - \tilde{\mu}_{i,\hat{\lambda}}$, $\hat{u}_{it} - \check{u}_{it}$, $\hat{\omega}_i - \check{\omega}_i$, and $\hat{h}_{it,\zeta,\hat{\omega}_i} - \check{h}_{it,\zeta,\check{\omega}_i}$. Similar to (2.2), $B_{\hat{\psi}}^{-1}(A_{\hat{\phi}} y_i - x_i\hat{\beta})$ can be rewritten as $(\hat{u}^*_{i1,\hat{\lambda}}, ..., \hat{u}^*_{iT,\hat{\lambda}})'$ with

$$\hat{u}^*_{it,\hat{\lambda}} = y_{it} - x_{it}'\hat{\beta} - \hat{\phi} y_{i,t-1} - \hat{\psi}\hat{u}^*_{i,t-1,\hat{\lambda}},$$

with the initial values $y_{i0} = \hat{u}^*_{i0,\hat{\lambda}} = 0$. Likewise, $(1+\hat{\psi}\mathcal{B})^{-1}(y_{it} - x_{it}'\hat{\beta} - \hat{\phi} y_{i,t-1})$ can be redefined as $(\tilde{u}^*_{iT,\hat{\lambda}}, ..., \tilde{u}^*_{iT,\hat{\lambda}})'$ with

$$\tilde{u}^*_{it,\hat{\lambda}} = y_{it} - x_{it}'\hat{\beta} - \hat{\phi} y_{i,t-1} - \hat{\psi}\tilde{u}^*_{i,t-1,\hat{\lambda}}.$$

Then, we have

$$\hat{u}^*_{it,\hat{\lambda}} - \tilde{u}^*_{it,\hat{\lambda}} = (-\hat{\psi})^t(\hat{\phi} y_{i0} + \hat{\psi}\tilde{u}^*_{i0,\hat{\lambda}}). \tag{C.28}$$

Denote $(l_T'\Sigma_{\hat{\psi}}^{-1} l_T)^{-1} l_T' B_{\hat{\psi}}'^{-1} := T^{-1}(w_{1,\hat{\psi}}, ..., w_{T,\hat{\psi}})$. By using the fact $\sum_{t=1}^{T} c^t \mathcal{Y}_t = O_p(1)$ with $|c| < 1$ and the variable $\mathcal{Y}_t$ satisfying $\mathrm{E}|\mathcal{Y}_t| < \infty$, $|\hat{\psi}| < 1$, and the $L_2$-boundedness of $\hat{u}^*_{it,\hat{\lambda}}$, it is not difficult to show

$$\frac{1}{T}\sum_{t=1}^{T}[w_{t,\hat{\psi}} - (1+\hat{\psi})]\hat{u}^*_{it,\hat{\lambda}} = O_p\Big(\frac{1}{T}\Big). \tag{C.29}$$

By (C.27)–(C.29), it follows that

$$\begin{aligned}&\hat{\mu}_{i,\hat{\lambda}} - \tilde{\mu}_{i,\hat{\lambda}}\\ &= \frac{1}{T}\sum_{t=1}^{T}[w_{t,\hat{\psi}} - (1+\hat{\psi})]\hat{u}^*_{it,\hat{\lambda}} + (1+\hat{\psi})\frac{1}{T}\sum_{t=1}^{T}(\hat{u}^*_{it,\hat{\lambda}} - \tilde{u}^*_{it,\hat{\lambda}})\\ &= O_p\Big(\frac{1}{T}\Big) + (1+\hat{\psi})\frac{1}{T}\sum_{t=1}^{T}(\hat{u}^*_{it,\hat{\lambda}} - \tilde{u}^*_{it,\hat{\lambda}}) = O_p\Big(\frac{1}{T}\Big).\end{aligned}$$

Back to (C.26), for each $i$ and $t$, we can show

$$\Delta_{2,it} := \hat{u}_{it} - \breve{u}_{it} = \frac{1-(-\hat{\psi})^{t-1}}{1+\hat{\psi}}(\tilde{\mu}_{i,\hat{\lambda}} - \hat{\mu}_{i,\hat{\lambda}}) + (-\hat{\psi})^{t-1}(\hat{\phi}y_{i0} + \hat{\psi}u_{i0}). \tag{C.30}$$

As $|\hat{\psi}| < 1$, it implies that

$$\hat{\omega}_i - \breve{\omega}_i = \frac{1}{T}\sum_{t=1}^{T}(\hat{u}_{i,t-1}^2 - \breve{u}_{i,t-1}^2) = \frac{1}{T}\sum_{t=1}^{T}(\Delta_{2,it}^2 + 2\Delta_{2,it}\breve{u}_{it}) = O_p\Big(\frac{1}{T}\Big). \tag{C.31}$$

Note that $\hat{h}_{it,\zeta,\hat{\omega}_i} - \breve{h}_{it,\zeta,\breve{\omega}_i} = (1-\tau-\nu)(\hat{\omega}_i - \breve{\omega}_i) + \tau(\hat{u}_{i,t-1}^2 - \breve{u}_{i,t-1}^2) + \nu(\hat{h}_{i,t-1,\zeta,\hat{\omega}_i} - \breve{h}_{i,t-1,\zeta,\breve{\omega}_i})$ with $c_h = \hat{h}_{i0,\zeta,\hat{\omega}_i}$. Then, we have

$$\begin{aligned}&\hat{h}_{it,\zeta,\hat{\omega}_i} - \breve{h}_{it,\zeta,\breve{\omega}_i} \\ &= \frac{1-\nu^t}{1-\nu}(1-\tau-\nu)(\hat{\omega}_i - \breve{\omega}_i) + \tau\sum_{t^*=1}^{t}\nu^{t^*-1}(\Delta_{2,i,t-t^*}^2 + 2\Delta_{2,i,t-t^*}\breve{u}_{i,t-t^*}) + \nu^t(c_h - \breve{h}_{i0,\zeta,\breve{\omega}_i}).\end{aligned} \tag{C.32}$$

Second, we consider $L_\zeta^\dagger = \hat{L}_{\zeta,\hat{\omega}} - \breve{L}_{\zeta,\breve{\omega}}$, which is given by

$$\frac{1}{NT}L_\zeta^\dagger = -\frac{1}{2NT}\sum_{i=1}^{N}\sum_{t=1}^{T}\Big\{\Big(\frac{\hat{u}_{it}^2}{\hat{h}_{it,\zeta,\hat{\omega}_i}} - \frac{\breve{u}_{it}^2}{\breve{h}_{it,\zeta,\breve{\omega}_i}}\Big) + [\log(\hat{h}_{it,\zeta,\hat{\omega}_i}) - \log(\breve{h}_{it,\zeta,\breve{\omega}_i})]\Big\}. \tag{C.33}$$

For the first term in the RHS of (C.33), we have

$$\begin{aligned}&\frac{1}{NT}\sum_{i=1}^{N}\sum_{t=1}^{T}\Big\{\frac{\hat{u}_{it}^2}{\hat{h}_{it,\zeta,\hat{\omega}_i}} - \frac{\breve{u}_{it}^2}{\breve{h}_{it,\zeta,\breve{\omega}_i}}\Big\} \\ &= \frac{1}{NT}\sum_{i=1}^{N}\sum_{t=1}^{T}\Big\{\frac{\hat{u}_{it}^2}{\hat{h}_{it,\zeta,\hat{\omega}_i}} - \frac{\breve{u}_{it}^2}{\hat{h}_{it,\zeta,\hat{\omega}_i}} + \frac{\breve{u}_{it}^2}{\hat{h}_{it,\zeta,\hat{\omega}_i}} - \frac{\breve{u}_{it}^2}{\breve{h}_{it,\zeta,\breve{\omega}_i}}\Big\} \\ &= \frac{1}{NT}\sum_{i=1}^{N}\sum_{t=1}^{T}\Big\{\frac{\Delta_{2,it}^2 + 2\Delta_{2,it}\breve{u}_{it}}{\hat{h}_{it,\zeta,\hat{\omega}_i}} + \frac{\breve{u}_{it}^2(\breve{h}_{it,\zeta,\breve{\omega}_i} - \hat{h}_{it,\zeta,\hat{\omega}_i})}{\hat{h}_{it,\zeta,\hat{\omega}_i}\breve{h}_{it,\zeta,\breve{\omega}_i}}\Big\} \\ &= O_p\Big(\frac{1}{T}\Big).\end{aligned} \tag{C.34}$$

To prove the last equation in (C.34), we note that $|\hat{\psi}|$ in $\Delta_{2,it}$ and $|\nu|$ in $\breve{h}_{it,\zeta,\breve{\omega}_i} - \hat{h}_{it,\zeta,\hat{\omega}_i}$ are smaller than 1, $u_{it}$ and $y_{it}$ are $L_4$-bounded, and $\hat{h}_{it,\zeta,\hat{\omega}_i}, \breve{h}_{it,\zeta,\breve{\omega}_i} > c^*$ with a positive constant $c^*$. Then, by (C.28)–(C.32), it is observed that the LHS of this equation can be further divided into some parts having the structure $(NT)^{-1}\sum_{i=1}^{N}\sum_{t=1}^{T}c^t\mathcal{Y}_{it}$ with $|c| < 1$ and the variable $\mathcal{Y}_{it}$ satisfying $\mathrm{E}|\mathcal{Y}_{it}| < \infty$. Hence, this equation holds by using the fact that $(NT)^{-1}\sum_{i=1}^{N}\sum_{t=1}^{T}c^t\mathcal{Y}_{it} = O(T^{-1})$ implied by the Markov's inequality.

For the second term in the RHS of (C.33), we suppose that $\log(\hat{h}_{it,\zeta,\hat{\omega}_i}) \geq \log(\check{h}_{it,\zeta,\check{\omega}_i})$ w.l.o.g. Then, we can show

$$\frac{1}{NT}\sum_{i=1}^{N}\sum_{t=1}^{T}[\log(\hat{h}_{it,\zeta,\hat{\omega}_i}) - \log(\check{h}_{it,\zeta,\check{\omega}_i})] = \frac{1}{NT}\sum_{i=1}^{N}\sum_{t=1}^{T}\log\left(1 + \frac{\hat{h}_{it,\zeta,\hat{\omega}_i} - \check{h}_{it,\zeta,\check{\omega}_i}}{\check{h}_{it,\zeta,\check{\omega}_i}}\right)$$

$$\leq \frac{1}{NT}\sum_{i=1}^{N}\sum_{t=1}^{T}\frac{\hat{h}_{it,\zeta,\hat{\omega}_i} - \check{h}_{it,\zeta,\check{\omega}_i}}{\check{h}_{it,\zeta,\check{\omega}_i}} = O_p\Big(\frac{1}{T}\Big),$$

where the inequality follows from the fact that $\log(1+x) \leq x$ for $x > 0$, and the term of $O_p(T^{-1})$ can be obtained as for (C.34). Back to (C.33), we have $(NT)^{-1}L_\zeta^\dagger = O_p(T^{-1}) = o_p(1)$. It means the initial values effect is negligible for the consistency. □

**Proof for Lemma C.8(ii).** As $L_\zeta^\S = \check{L}_{\zeta,\check{\omega}} - \tilde{L}_{\zeta,\tilde{\omega}}$, we have

$$\frac{1}{NT}L_\zeta^\S = -\frac{1}{2NT}\sum_{i=1}^{N}\sum_{t=1}^{T}\Big\{\Big(\frac{\check{u}_{it}^2}{\check{h}_{it,\zeta,\check{\omega}_i}} - \frac{\tilde{u}_{it}^2}{\tilde{h}_{it,\zeta,\tilde{\omega}_i}}\Big) + [\log(\check{h}_{it,\zeta,\check{\omega}_i}) - \log(\tilde{h}_{it,\zeta,\tilde{\omega}_i})]\Big\}. \quad \text{(C.35)}$$

Recall that

$$\check{u}_{it} = y_{it} - \tilde{\mu}_{i,\hat{\lambda}} - x_{it}'\hat{\beta} - \sum_{p=1}^{P}\hat{\phi}_p y_{i,t-p} - \sum_{q=1}^{Q}\hat{\psi}_q \check{u}_{i,t-q,\hat{\lambda}},$$
$$\tilde{u}_{it} = y_{it} - \tilde{\mu}_{i,\lambda_0} - x_{it}'\beta_0 - \sum_{p=1}^{P}\phi_{0p} y_{i,t-p} - \sum_{q=1}^{Q}\psi_{0q}\tilde{u}_{i,t-q}, \quad \text{(C.36)}$$

where $\tilde{\mu}_{i,\lambda} = (1+\psi)T^{-1}\sum_{t=1}^{T}(1+\psi\mathcal{B})^{-1}(y_{it} - x_{it}'\beta - \phi y_{i,t-1})$. By using Taylor's expansion with respect to $\lambda$ (see the similar discussions in (C.43) below) and (C.22), it is not difficult to show

$$\frac{1}{2NT}\sum_{i=1}^{N}\sum_{t=1}^{T}\Big\{\Big(\frac{\check{u}_{it}^2}{\check{h}_{it,\zeta,\check{\omega}_i}} - \frac{\tilde{u}_{it}^2}{\tilde{h}_{it,\zeta,\tilde{\omega}_i}}\Big) + [\log(\check{h}_{it,\zeta,\check{\omega}_i}) - \log(\tilde{h}_{it,\zeta,\tilde{\omega}_i})]\Big\} = O_p\Big(\max\Big(\frac{1}{\sqrt{NT}}, \frac{1}{T}\Big)\Big).$$

Back to (C.35), we have $(NT)^{-1}L_\zeta^\S = o_p(1)$. It means that the estimation effect of $\lambda_0$ is negligible for the consistency. □

**Proof for Lemma C.8(iii).** As $L_\zeta^\sharp = \tilde{L}_{\zeta,\tilde{\omega}} - \bar{L}_{\zeta,\bar{\omega}}$, we have

$$\frac{1}{NT}L_\zeta^\sharp = -\frac{1}{2NT}\sum_{i=1}^{N}\sum_{t=1}^{T}\Big\{\Big(\frac{\tilde{u}_{it}^2}{\tilde{h}_{it,\zeta,\tilde{\omega}_i}} - \frac{u_{it}^2}{h_{it,\zeta,\bar{\omega}_i}}\Big) + [\log(\tilde{h}_{it,\zeta,\tilde{\omega}_i}) - \log(h_{it,\zeta,\bar{\omega}_i})]\Big\}.$$

Similar to (C.30)–(C.32), it is obtained that

$$\tilde{u}_{it} - u_{it} = -\frac{1}{T}\sum_{t=1}^{T} u_{it} = O_p\Big(\frac{1}{\sqrt{T}}\Big), \qquad \tilde{\omega}_i - \bar{\omega}_i = -\Big(\frac{1}{T}\sum_{t=1}^{T} u_{it}\Big)^2 = O_p\Big(\frac{1}{T}\Big),$$

$$\begin{aligned}\tilde{h}_{it,\zeta,\tilde{\omega}_i} - h_{it,\zeta,\bar{\omega}_i} &= \frac{1-\nu^t}{1-\nu}\Big[(1-\tau-\nu)(\tilde{\omega}_i - \bar{\omega}_i) + \tau\Big(\frac{1}{T}\sum_{t=1}^{T} u_{it}\Big)^2\Big] \\ &\quad - 2\tau\sum_{t^*=1}^{t}\nu^{t^*-1}u_{i,t-t^*}\Big(\frac{1}{T}\sum_{t=1}^{T} u_{it}\Big) + \nu^t(\tilde{h}_{i0,\zeta,\tilde{\omega}_i} - h_{i0,\zeta,\bar{\omega}_i}).\end{aligned} \tag{C.37}$$

Using similar arguments as for $L_\zeta^\dagger$, we can show that $(NT)^{-1}L_\zeta^\sharp = O_p(1/\sqrt{T}) = o_p(1)$. It indicates that the estimation effect of $\mu_0$ is negligible for the consistency. □

**Proof for Lemma C.8(iv).** As $L_\zeta^\flat = \bar{L}_{\zeta,\bar{\omega}} - L_{\zeta,\omega_0}$, we have

$$\frac{1}{NT}L_\zeta^\flat = -\frac{1}{2NT}\sum_{i=1}^{N}\sum_{t=1}^{T}\Big\{\Big(\frac{u_{it}^2}{h_{it,\zeta,\bar{\omega}_i}} - \frac{u_{it}^2}{h_{it,\zeta,\omega_0}}\Big) + [\log(h_{it,\zeta,\bar{\omega}_i}) - \log(h_{it,\zeta,\omega_0})]\Big\}.$$

By (C.25), we have $u_{it}^2 = \omega_{0i}(1-\kappa_0) + \kappa_0 u_{i,t-1}^2 + (u_{it}^2 - h_{it}) - \nu_0(u_{i,t-1}^2 - h_{i,t-1})$. Hence,

$$\begin{aligned}&\bar{\omega}_i - \omega_{0i} \\ &= (1-\kappa_0)^{-1}\Big[(1-\nu_0)\frac{1}{T}\sum_{t=1}^{T}(u_{it}^2 - h_{it}) + \kappa_0\frac{1}{T}(u_{i0}^2 - u_{iT}^2) + \nu_0\frac{1}{T}(u_{iT}^2 - h_{iT} - u_{i0}^2 + h_{i0})\Big] \\ &= (1-\kappa_0)^{-1}(1-\nu_0)\frac{1}{T}\sum_{t=1}^{T}(u_{it}^2 - h_{it}) + O_p\Big(\frac{1}{T}\Big).\end{aligned} \tag{C.38}$$

Like (C.30), we can show

$$\begin{aligned}h_{it,\zeta,\bar{\omega}_i} - h_{it,\zeta,\omega_{0i}} &= \frac{1-\kappa}{1-\nu}(\bar{\omega}_i - \omega_{0i}) = \frac{(1-\kappa)(1-\nu_0)}{(1-\nu)(1-\kappa_0)}\frac{1}{T}\sum_{t=1}^{T}(u_{it}^2 - h_{it}) + O_p\Big(\frac{1}{T}\Big) \\ &= O_p\Big(\frac{1}{\sqrt{T}}\Big).\end{aligned} \tag{C.39}$$

By using similar ideas as for $L_\zeta^\dagger$, we have $(NT)^{-1}L_\zeta^\flat = O_p(1/\sqrt{T}) = o_p(1)$. It illustrates that the estimation effect of $\omega_0$ is negligible for the consistency. □

Since we need to provide the exact expressions for the asymptotic distribution, we give the proof of Claim C.9 based on the general panel ARMA$(P,Q)$–GARCH$(L,K)$ model.

**Proof for Claim C.9(i).** By (B.6), it is given that

$$\frac{1}{\sqrt{NT}}G^\dagger = \frac{1}{2\sqrt{NT}}\sum_{i=1}^{N}\sum_{t=1}^{T}\Big(\frac{\hat{u}_{it}^2 - \hat{h}_{it,\zeta_0,\hat{\omega}_i}}{\hat{h}_{it,\zeta_0,\hat{\omega}_i}^2}\frac{\partial\hat{h}_{it,\zeta_0,\hat{\omega}_i}}{\partial\zeta} - \frac{\check{u}_{it}^2 - \check{h}_{it,\zeta_0,\check{\omega}_i}}{\check{h}_{it,\zeta_0,\check{\omega}_i}^2}\frac{\partial\check{h}_{it,\zeta_0,\check{\omega}_i}}{\partial\zeta}\Big),$$

where $\partial h_{it,\zeta_0,\omega_i}/\partial\zeta$ is a linear function of $u_{it}^2$ and $\omega_i$ by (B.9). Then, we aim to prove

$$\frac{1}{\sqrt{NT}}G^\dagger = \frac{1}{\sqrt{NT}}\mathrm{E}(G^\dagger) + o_p\Big(\sqrt{\frac{N}{T}}\Big) = \frac{1}{\sqrt{NT}}\Delta^\dagger + o_p\Big(\sqrt{\frac{N}{T}}\Big), \tag{C.40}$$

where $\Delta^\dagger = \mathrm{E}(G^\dagger) = O(N)$, whose exact expression is unavailable. From (C.40), we know that the initial values impose an asymptotic bias on the asymptotic distribution of $\hat{\zeta}$.

Like (C.34), $G^\dagger$ can be divided into several parts having the structure $\sum_{i=1}^N \sum_{t=1}^T c^t \mathcal{Y}_{it}$ with $|c| < 1$ and $\mathrm{E}|\mathcal{Y}_{it}| < \infty$. To prove (C.40), it suffices to show

$$\frac{1}{N}\sum_{i=1}^N \sum_{t=1}^T c^t[\mathcal{Y}_{it} - \mathrm{E}(\mathcal{Y}_{it})] = o_p(1), \tag{C.41}$$

which holds if

$$\begin{aligned}
&(i)\ \frac{1}{N}\sum_{i=1}^N \sum_{t=1}^C c^t[\mathcal{Y}_{it} - \mathrm{E}(\mathcal{Y}_{it})] = o_p(1), \quad \forall C \geq 1;\\
&(ii)\ \frac{1}{N}\sum_{i=1}^N \sum_{t=C+1}^T c^t \mathrm{E}|\mathcal{Y}_{it} - \mathrm{E}(\mathcal{Y}_{it})| \to 0, \quad \text{as } N, T, C \to \infty.
\end{aligned} \tag{C.42}$$

For (i) in (C.42), it is a direct result of the law of large number for independent variables; see Theorem 5.4.1. in Chung (2001). For (ii) in (C.42), as $N, T, C \to \infty$, we have

$$\frac{1}{N}\sum_{i=1}^N \sum_{t=C+1}^T c^t \mathrm{E}|\mathcal{Y}_{it} - \mathrm{E}(\mathcal{Y}_{it})| = c^C \frac{1}{N}\sum_{i=1}^N \sum_{t=C+1}^T c^{t-C} \mathrm{E}|\mathcal{Y}_{it} - \mathrm{E}(\mathcal{Y}_{it})| = o(1),$$

where the last equation holds since $|c| < 1$ and $\mathcal{Y}_{it}$ is $L_1$-bounded. Hence, (C.41) holds. □

**Proof for Claim C.9(ii).** As $G^\S = \check{G} - \tilde{G}$, we have

$$\frac{1}{\sqrt{NT}}G^\S = \frac{1}{2\sqrt{NT}}\sum_{i=1}^N \sum_{t=1}^T \Big(\frac{\check{u}_{it}^2 - \check{h}_{it,\zeta_0,\check{\omega}_i}}{\check{h}_{it,\zeta_0,\check{\omega}_i}^2}\frac{\partial \check{h}_{it,\zeta_0,\check{\omega}_i}}{\partial\zeta} - \frac{\tilde{u}_{it}^2 - \tilde{h}_{it,\zeta_0,\tilde{\omega}_i}}{\tilde{h}_{it,\zeta_0,\tilde{\omega}_i}^2}\frac{\partial \tilde{h}_{it,\zeta_0,\tilde{\omega}_i}}{\partial\zeta}\Big),$$

where $\check{u}_{it}$ and $\tilde{u}_{it}$ are given in (C.36). Denote

$$\tilde{G}_\lambda = \frac{1}{2}\sum_{i=1}^N \sum_{t=1}^T \frac{\tilde{u}_{it,\lambda}^2 - \tilde{h}_{it,\zeta_0,\lambda}}{\tilde{h}_{it,\zeta_0,\lambda}^2}\frac{\partial \tilde{h}_{it,\zeta_0,\lambda}}{\partial\zeta},$$

where $\tilde{h}_{it,\zeta_0,\lambda}$ is based on $\tilde{u}_{it,\lambda}^2$. Then, $\tilde{G}_{\lambda_0} = \tilde{G}$. By Taylor's expansion with respect to $\lambda$, we have

$$\frac{1}{\sqrt{NT}}G^\S = \Pi^* \times \sqrt{NT}(\hat{\lambda} - \lambda_0), \tag{C.43}$$

where $\Pi^* = (NT)^{-1}\partial\tilde{G}_{\lambda^*}/\partial\lambda$ is a $(L+K)\times(D_x+P+Q)$–dimensional matrix, and $\lambda^* \in \Theta_\lambda$ lies between $\hat{\lambda}$ and $\lambda_0$. Similar to (C.21), we can show

$$\Pi^* = \frac{1}{NT}\frac{\partial\tilde{G}}{\partial\lambda} + O_p\Big(\max\Big(\frac{1}{\sqrt{NT}}, \frac{1}{T}\Big)\Big). \tag{C.44}$$

Next, we aim to prove

$$\frac{1}{NT}\frac{\partial\tilde{G}}{\partial\lambda} = \Pi + O_p\Big(\frac{1}{\sqrt{T}}\Big). \tag{C.45}$$

Let $x^*_{it,d_x} = x_{it,d_x} - \mathrm{E}(x_{it,d_x})$. For the $(l, d_x)$-th element of $\partial\tilde{G}/\partial\lambda$, it is observed that

$$\begin{aligned}
&\frac{1}{2NT}\sum_{i=1}^{N}\sum_{t=1}^{T}\frac{\partial(\tilde{u}_{it}^2 - \tilde{h}_{it,\zeta_0,\tilde{\omega}_i})\tilde{h}^{-2}_{it,\zeta_0,\tilde{\omega}_i}(\partial\tilde{h}_{it,\zeta_0,\tilde{\omega}_i}/\partial\tau_l)}{\partial\beta_{d_x}}\\
&= \frac{1}{2NT}\sum_{i=1}^{N}\sum_{t=1}^{T}\frac{(-2\tilde{u}_{it}^2 + \tilde{h}_{it,\zeta_0,\tilde{\omega}_i})}{\tilde{h}^3_{it,\zeta_0,\tilde{\omega}_i}}\frac{\partial\tilde{h}_{it,\zeta_0,\tilde{\omega}_i}}{\partial\tau_l}\frac{\partial\tilde{h}_{it,\zeta_0,\tilde{\omega}_i}}{\partial\beta_{d_x}}\\
&\quad + \frac{1}{2NT}\sum_{i=1}^{N}\sum_{t=1}^{T}\frac{2\tilde{u}_{it}}{\tilde{h}^2_{it,\zeta_0,\tilde{\omega}_i}}\frac{\partial\tilde{h}_{it,\zeta_0,\tilde{\omega}_i}}{\partial\tau_l}\frac{\partial\tilde{u}_{it}}{\partial\beta_{d_x}} + \frac{1}{2NT}\sum_{i=1}^{N}\sum_{t=1}^{T}\frac{(\tilde{u}_{it}^2 - \tilde{h}_{it,\zeta_0,\tilde{\omega}_i})}{\tilde{h}^2_{it,\zeta_0,\tilde{\omega}_i}}\frac{\partial^2\tilde{h}_{it,\zeta_0,\tilde{\omega}_i}}{\partial\tau_l\partial\beta_{d_x}}\\
&= -\frac{1}{2NT}\sum_{i=1}^{N}\sum_{t=1}^{T}\frac{1}{h_{it}^2}\frac{\partial h_{it}}{\partial\tau_l}\frac{\partial\tilde{h}_{it,\zeta_0,\omega_0}}{\partial\beta_{d_x}} + O_p\Big(\frac{1}{\sqrt{T}}\Big) + O_p\Big(\frac{1}{\sqrt{T}}\Big)\\
&= \frac{1}{2NT}\sum_{i=1}^{N}\sum_{t=1}^{T}\frac{1}{h_{it}^2}\frac{\partial h_{it}}{\partial\tau_l}\Big[\Big(1 - \sum_{k=1}^{K}\nu_{0k}\mathcal{B}^k\Big)^{-1}\Big(\sum_{l=1}^{L}\tau_{0l}\mathcal{B}^l\Big)2u_{it}\Big]\Big[\Big(1 + \sum_{q=1}^{Q}\psi_{0q}\mathcal{B}^q\Big)x^*_{it,d_x}\Big]\\
&\quad + O_p\Big(\frac{1}{\sqrt{T}}\Big),
\end{aligned}$$

where the second equation follows from the fact that $\tilde{u}_{it} - u_{it} = O_p(1/\sqrt{T})$ and $\tilde{h}_{it,\zeta,\tilde{\omega}_i} - h_{it} = O_p(1/\sqrt{T})$ as for (C.52) below. Note that the first item in the RHS of the last equation is the $(l, d_x)$-th element of $\Pi$ in (B.11). Hence, (C.45) holds for the $(l, d_x)$-th element of $\partial\tilde{G}/\partial\lambda$. Similarly, we can show that (C.45) holds for other elements of $\partial\tilde{G}/\partial\lambda$.

By (C.44)–(C.45), we know

$$\Pi^* = \Pi + O_p\Big(\frac{1}{\sqrt{T}}\Big).$$

Back to (C.43), by (C.23), it follows that

$$\frac{1}{\sqrt{NT}}G^{\S} = \frac{1}{\sqrt{NT}}\Pi\Gamma_1^{-1}[D - \mathrm{E}(D)] + \frac{1}{\sqrt{NT}}\Delta^{\S} + O_p\Big(\frac{1}{\sqrt{T}}\Big),$$

where

$$\Delta^{\S} = \Pi\Gamma_1^{-1}[\mathrm{E}(D) + \mathrm{E}(D^\dagger)]. \tag{C.46}$$

It means that the estimation effect of $\lambda_0$ has an impact on the asymptotic bias and variance of $\hat{\zeta}$. $\square$

**Proof for Claim C.9(iii).** As $G^\sharp = \tilde{G} - \bar{G}$, we have

$$\frac{1}{\sqrt{NT}} G^\sharp = \frac{1}{2\sqrt{NT}} \sum_{i=1}^{N} \sum_{t=1}^{T} \Big( \frac{\tilde{u}_{it}^2 - \tilde{h}_{it,\zeta_0,\tilde{\omega}_i}}{\tilde{h}_{it,\zeta_0,\tilde{\omega}_i}^2} \frac{\partial \tilde{h}_{it,\zeta_0,\tilde{\omega}_i}}{\partial \zeta} - \frac{u_{it}^2 - h_{it,\zeta_0,\bar{\omega}_i}}{h_{it,\zeta_0,\bar{\omega}_i}^2} \frac{\partial h_{it,\zeta_0,\bar{\omega}_i}}{\partial \zeta} \Big). \tag{C.47}$$

Since $\tilde{u}_{it}^2 - \tilde{\omega}_i = u_{it}^2 - \bar{\omega}_i - 2u_{it}(\sum_{t=1}^T u_{it})/T$, by (B.8)–(B.9), it follows that

$$\begin{aligned}
&\frac{1}{2NT} \sum_{i=1}^{N} \sum_{t=1}^{T} \frac{\tilde{u}_{it}^2 - \tilde{h}_{it,\zeta_0,\tilde{\omega}_i}}{h_{it}^2} \frac{\partial \tilde{h}_{it,\zeta_0,\tilde{\omega}_i}}{\partial \tau_l} \\
&= \frac{1}{2NT} \sum_{i=1}^{N} \sum_{t=1}^{T} h_{it}^{-2} \Big[ \Big(1 - \sum_{k=1}^{K} \nu_{0k} \mathcal{B}^k \Big)^{-1} \Big(1 - \sum_{k=1}^{K} \kappa_{0k} \mathcal{B}^k \Big) (\tilde{u}_{it}^2 - \tilde{\omega}_i) \Big] \\
&\quad \times \Big[ \big(1 - \sum_{k=1}^{K} \nu_{0k} \mathcal{B}^k \big)^{-1} \mathcal{B}^l (\tilde{u}_{it}^2 - \tilde{\omega}_i) \Big] \\
&:= \frac{1}{2NT} \sum_{i=1}^{N} \sum_{t=1}^{T} (\mathcal{O}_{1,it} + \mathcal{O}_{2,it}) \times (\mathcal{O}_{3,it,l} + \mathcal{O}_{4,it,l}),
\end{aligned} \tag{C.48}$$

where

$$\begin{aligned}
\mathcal{O}_{1,it} &= h_{it}^{-1} \Big[ \Big(1 - \sum_{k=1}^{K} \nu_{0k} \mathcal{B}^k \Big)^{-1} \Big(1 - \sum_{k=1}^{K} \kappa_{0k} \mathcal{B}^k \Big) (u_{it}^2 - \bar{\omega}_i) \Big], \\
\mathcal{O}_{2,it} &= -2h_{it}^{-1} \Big[ \Big(1 - \sum_{k=1}^{K} \nu_{0k} \mathcal{B}^k \Big)^{-1} \Big(1 - \sum_{k=1}^{K} \kappa_{0k} \mathcal{B}^k \Big) u_{it} \Big] \Big( \frac{1}{T} \sum_{t=1}^{T} u_{it} \Big), \\
\mathcal{O}_{3,it,l} &= h_{it}^{-1} \Big[ \Big(1 - \sum_{k=1}^{K} \nu_{0k} \mathcal{B}^k \Big)^{-1} \mathcal{B}^l (u_{it}^2 - \bar{\omega}_i) \Big], \\
\mathcal{O}_{4,it,l} &= -2h_{it}^{-1} \Big[ \Big(1 - \sum_{k=1}^{K} \nu_{0k} \mathcal{B}^k \Big)^{-1} \mathcal{B}^l u_{it} \Big] \Big( \frac{1}{T} \sum_{t=1}^{T} u_{it} \Big).
\end{aligned}$$

Below, we analyze $\mathcal{O}_{1,it} \times \mathcal{O}_{3,it,l}$, $\mathcal{O}_{1,it} \times \mathcal{O}_{4,it,l}$, $\mathcal{O}_{2,it} \times \mathcal{O}_{3,it,l}$, and $\mathcal{O}_{2,it} \times \mathcal{O}_{4,it,l}$ one by one.

First, by (C.61) below, we have

$$\frac{1}{2NT} \sum_{i=1}^{N} \sum_{t=1}^{T} \mathcal{O}_{1,it} \times \mathcal{O}_{3,it,l} = \frac{1}{2NT} \sum_{i=1}^{N} \sum_{t=1}^{T} \frac{u_{it}^2 - h_{it,\zeta_0,\bar{\omega}_i}}{h_{it,\zeta_0,\bar{\omega}_i}^2} \frac{\partial h_{it,\zeta_0,\bar{\omega}_i}}{\partial \tau_l} - \frac{1}{NT} \Delta_{3,\tau_l}^\flat + o_p\Big(\frac{1}{T}\Big),$$

where

$$\Delta_{3,\tau_l}^\flat = -\sum_{i=1}^{N} \Big[ \mathrm{E}\Big( \frac{1}{h_{it}} \frac{\partial h_{it}}{\partial \tau_l} \Big) - \mathrm{E}\Big( \frac{1}{h_{it}^3} \frac{\partial h_{it}}{\partial \tau_l} \Big) \mathrm{E}(h_{it}^2) \Big] [\mathrm{E}(\epsilon_{it}^4) - 1].$$

Second, we can show

$$
\begin{aligned}
&\frac{1}{N}\sum_{i=1}^{N}\Big(\frac{1}{\sqrt{T}}\sum_{t=1}^{T}(u_{it}^2-h_{it})\Big)\Big(\frac{1}{\sqrt{T}}\sum_{t=1}^{T}u_{it}\Big)\\
&=\frac{1}{2N}\sum_{i=1}^{N}\Big[\Big(\frac{1}{\sqrt{T}}\sum_{t=1}^{T}(u_{it}^2-h_{it}+u_{it})\Big)^2-\Big(\frac{1}{\sqrt{T}}\sum_{t=1}^{T}(u_{it}^2-h_{it})\Big)^2-\Big(\frac{1}{\sqrt{T}}\sum_{t=1}^{T}u_{it}\Big)^2\Big]\\
&=\frac{1}{2N}\sum_{i=1}^{N}\mathrm{E}\Big[\Big(\frac{1}{\sqrt{T}}\sum_{t=1}^{T}(u_{it}^2-h_{it}+u_{it})\Big)^2-\Big(\frac{1}{\sqrt{T}}\sum_{t=1}^{T}(u_{it}^2-h_{it})\Big)^2-\Big(\frac{1}{\sqrt{T}}\sum_{t=1}^{T}u_{it}\Big)^2\Big]+o_p(1)\\
&=\frac{1}{NT}\sum_{i=1}^{N}\mathrm{E}\big[(u_{it}^2-h_{it})u_{it}\big]+o_p(1), \qquad (C.49)
\end{aligned}
$$

where the first equation comes from the fact that $ab=[(a+b)^2-a^2-b^2]/2$, and the second equation follows from Theorem 1 in Phillips and Moon (1999) by using the $L_4$-boundedness of $u_{it}$, the martingale difference CLT, and continuous mapping theorem. Then, it yields

$$
\begin{aligned}
&\frac{1}{2NT}\sum_{i=1}^{N}\sum_{t=1}^{T}\mathcal{O}_{1,it}\times\mathcal{O}_{4,it,l}\\
&=-\frac{1}{NT}\sum_{i=1}^{N}\sum_{t=1}^{T}h_{it}^{-2}(u_{it}^2-h_{it}+h_{it}-h_{it,\zeta_0,\bar{\omega}_i})\Big[\Big(1-\sum_{k=1}^{K}\nu_{0k}\mathcal{B}^k\Big)^{-1}\mathcal{B}^l u_{it}\Big]\Big(\frac{1}{T}\sum_{t=1}^{T}u_{it}\Big)\\
&=-\frac{1}{NT}\sum_{i=1}^{N}\frac{1}{\sqrt{T}}\sum_{t=1}^{T}h_{it}^{-2}(u_{it}^2-h_{it})\Big[\Big(1-\sum_{k=1}^{K}\nu_{0k}\mathcal{B}^k\Big)^{-1}\mathcal{B}^l u_{it}\Big]\Big(\frac{1}{\sqrt{T}}\sum_{t=1}^{T}u_{it}\Big)\\
&\quad+\frac{1}{NT}\sum_{i=1}^{N}\frac{1}{T}\sum_{t=1}^{T}h_{it}^{-2}\Big[\Big(1-\sum_{k=1}^{K}\nu_{0k}\mathcal{B}^k\Big)^{-1}\mathcal{B}^l u_{it}\Big]\Big(\frac{1}{\sqrt{T}}\sum_{t=1}^{T}(u_{it}^2-h_{it})\Big)\Big(\frac{1}{\sqrt{T}}\sum_{t=1}^{T}u_{it}\Big)+o_p\Big(\frac{1}{T}\Big)\\
&=\frac{1}{NT}\Delta_{1,\tau_l}^{\sharp}+o_p\Big(\frac{1}{T}\Big),
\end{aligned}
$$

where the second equation follows from (C.39), the third equation holds by (C.49), and

$$
\begin{aligned}
\Delta_{1,\tau_l}^{\sharp}=&-\sum_{i=1}^{N}\mathrm{E}\Big\{h_{it}^{-2}(u_{it}^2-h_{it})\Big[\Big(1-\sum_{k=1}^{K}\nu_{0k}\mathcal{B}^k\Big)^{-1}\mathcal{B}^l u_{it}\Big]u_{it}\Big\}\\
&+\sum_{i=1}^{N}\mathrm{E}\Big\{h_{it}^{-2}\Big[\Big(1-\sum_{k=1}^{K}\nu_{0k}\mathcal{B}^k\Big)^{-1}\mathcal{B}^l u_{it}\Big]\Big\}\mathrm{E}\big[(u_{it}^2-h_{it})u_{it}\big].
\end{aligned}
$$

Third, we write

$$
\frac{1}{2NT}\sum_{i=1}^{N}\sum_{t=1}^{T}\mathcal{O}_{2,it}\times\mathcal{O}_{3,it,l}:=\frac{1}{2NT}\sum_{i=1}^{N}\sum_{t=1}^{T}(\mathcal{O}_{23,it,l}^{\sharp}+\mathcal{O}_{23,it}^{\sharp\sharp})\Big(\frac{1}{T}\sum_{t=1}^{T}u_{it}\Big), \qquad (C.50)
$$

where

$$\mathcal{O}^{\sharp}_{23,it,l} = -2h_{it}^{-2}\Big[\Big(1-\sum_{k=1}^{K}\nu_{0k}\mathcal{B}^k\Big)^{-1}\Big(1-\sum_{k=1}^{K}\kappa_{0k}\mathcal{B}^k\Big)u_{it}\Big]\Big[\Big(1-\sum_{k=1}^{K}\nu_{0k}\mathcal{B}^k\Big)^{-1}\mathcal{B}^l(u_{it}^2-\omega_{0i})\Big],$$

$$\mathcal{O}^{\sharp\sharp}_{23,it} = -2h_{it}^{-2}\Big[\Big(1-\sum_{k=1}^{K}\nu_{0k}\mathcal{B}^k\Big)^{-1}\Big(1-\sum_{k=1}^{K}\kappa_{0k}\mathcal{B}^k\Big)u_{it}\Big]\Big[\Big(1-\sum_{k=1}^{K}\nu_{0k}\Big)^{-1}(\omega_{0i}-\bar{\omega}_i)\Big].$$

Using a similar idea as for (C.49), we have

$$\frac{1}{2NT}\sum_{i=1}^{N}\frac{1}{T}\sum_{t=1}^{T}\mathcal{O}^{\sharp}_{23,it,l}\Big(\sum_{t=1}^{T}u_{it}\Big) = \frac{1}{2NT}\sum_{i=1}^{N}\sum_{t=1}^{T}\mathrm{E}(\mathcal{O}^{\sharp}_{23,it,l})u_{it} + o_p\Big(\frac{1}{T}\Big),$$

and

$$\begin{aligned}
&\frac{1}{2NT}\sum_{i=1}^{N}\sum_{t=1}^{T}\mathcal{O}^{\sharp\sharp}_{23,it}\Big(\frac{1}{T}\sum_{t=1}^{T}u_{it}\Big)\\
&= \frac{1}{NT}\sum_{i=1}^{N}\frac{1}{T}\sum_{t=1}^{T}h_{it}^{-2}\Big[\Big(1-\sum_{k=1}^{K}\nu_{0k}\mathcal{B}^k\Big)^{-1}\Big(1-\sum_{k=1}^{K}\kappa_{0k}\mathcal{B}^k\Big)u_{it}\Big]\\
&\quad\times\Big(1-\sum_{k=1}^{K}\kappa_{0k}\Big)^{-1}\Big(\frac{1}{\sqrt{T}}\sum_{t=1}^{T}(u_{it}^2-h_{it})\Big)\Big(\frac{1}{\sqrt{T}}\sum_{t=1}^{T}u_{it}\Big)\\
&= \frac{1}{NT}\Delta^{\sharp}_{2,\tau_l} + o_p\Big(\frac{1}{T}\Big),
\end{aligned}$$

where the first equation follows from (C.38), and

$$\begin{aligned}
\Delta^{\sharp}_{2,\tau_l} = \sum_{i=1}^{N}\mathrm{E}\Big\{h_{it}^{-2}\Big[\Big(1-\sum_{k=1}^{K}\nu_{0k}\mathcal{B}^k\Big)^{-1}\Big(1-\sum_{k=1}^{K}\kappa_{0k}\mathcal{B}^k\Big)u_{it}\Big]\Big\}\\
\times\Big(1-\sum_{k=1}^{K}\kappa_{0k}\Big)^{-1}\mathrm{E}\big[(u_{it}^2-h_{it})u_{it}\big].
\end{aligned}$$

By (C.50), it follows that

$$\frac{1}{2NT}\sum_{i=1}^{N}\sum_{t=1}^{T}\mathcal{O}_{2,it}\times\mathcal{O}_{3,it,l} = \frac{1}{2NT}\sum_{i=1}^{N}\sum_{t=1}^{T}\mathrm{E}(\mathcal{O}^{\sharp}_{23,it,l})u_{it} + \frac{1}{NT}\Delta^{\sharp}_{2,\tau_l} + o_p\Big(\frac{1}{T}\Big).$$

Fourth, similar to (C.49), we can obtain

$$\begin{aligned}
&\frac{1}{2NT}\sum_{i=1}^{N}\sum_{t=1}^{T}\mathcal{O}_{2,it}\times\mathcal{O}_{4,it,l}\\
&= \frac{2}{NT}\sum_{i=1}^{N}\frac{1}{T}\sum_{t=1}^{T}h_{it}^{-2}\Big[\Big(1-\sum_{k=1}^{K}\nu_{0k}\mathcal{B}^k\Big)^{-1}\Big(1-\sum_{k=1}^{K}\kappa_{0k}\mathcal{B}^k\Big)u_{it}\Big]\Big[\Big(1-\sum_{k=1}^{K}\nu_{0k}\mathcal{B}^k\Big)^{-1}\mathcal{B}^l u_{it}\Big]
\end{aligned}$$

$$\times \Big(\frac{1}{\sqrt{T}}\sum_{t=1}^{T} u_{it}\Big)^2$$
$$= \frac{1}{NT}\Delta^{\sharp}_{3,\tau_l} + o_p\Big(\frac{1}{T}\Big),$$

where

$$\Delta^{\sharp}_{3,\tau_l} = 2\sum_{i=1}^{N} \mathrm{E}\Big\{h_{it}^{-2}\Big[\Big(1-\sum_{k=1}^{K}\nu_{0k}\mathcal{B}^k\Big)^{-1}\Big(1-\sum_{k=1}^{K}\kappa_{0k}\mathcal{B}^k\Big)u_{it}\Big]\Big[\Big(1-\sum_{k=1}^{K}\nu_{0k}\mathcal{B}^k\Big)^{-1}\mathcal{B}^l u_{it}\Big]\Big\}$$
$$\times \mathrm{E}(u_{it}^2).$$

Now, by (C.48), it follows that

$$\frac{1}{2NT}\sum_{i=1}^{N}\sum_{t=1}^{T}\Big(\frac{\tilde{u}_{it}^2-\tilde{h}_{it,\zeta_0,\tilde{\omega}_i}}{h_{it}^2}\frac{\partial \tilde{h}_{it,\zeta_0,\tilde{\omega}_i}}{\partial \tau_l} - \frac{u_{it}^2-h_{it,\zeta_0,\bar{\omega}_i}}{h_{it,\zeta_0,\bar{\omega}_i}^2}\frac{\partial h_{it,\zeta_0,\bar{\omega}_i}}{\partial \tau_l}\Big) \tag{C.51}$$
$$= \frac{1}{2NT}\sum_{i=1}^{N}\sum_{t=1}^{T}\mathrm{E}(\mathcal{O}^{\sharp}_{23,it,l})u_{it} + \frac{1}{NT}(\Delta^{\sharp}_{1,\tau_l}+\Delta^{\sharp}_{2,\tau_l}+\Delta^{\sharp}_{3,\tau_l}-\Delta^{\flat}_{3,\tau_l}) + o_p\Big(\frac{1}{T}\Big).$$

Next, we denote $\Delta_{h,it} := \tilde{h}_{it,\zeta_0,\tilde{\omega}_i} - h_{it}$. By (C.37) and (C.39), it is obtained that

$$\Delta_{h,it} = (\tilde{h}_{it,\zeta_0,\tilde{\omega}_i} - h_{it,\zeta_0,\bar{\omega}_i}) + (h_{it,\zeta_0,\bar{\omega}_i} - h_{it}) \tag{C.52}$$
$$= c_{it}\Big(\frac{1}{T}\sum_{t=1}^{T}u_{it}\Big) + \frac{1}{T}\sum_{t=1}^{T}(u_{it}^2-h_{it}) + O_p(c^t) + O_p\Big(\frac{1}{T}\Big)$$
$$:= \Delta^{*}_{h,it} + \Delta^{**}_{h,it} + O_p(c^t) + O_p\Big(\frac{1}{T}\Big),$$

where $c_{it} = -2\sum_{t^*=1}^{t}(\sum_{l=1}^{L}\tau_l\mathcal{B}^l)(\sum_{k=1}^{K}\nu_k\mathcal{B}^k)^{t^*-1}u_{i,t-t^*}$ and $|c|<1$. By Taylor's expansion, we have

$$\tilde{h}^{-2}_{it,\zeta_0,\tilde{\omega}_i} - h_{it}^{-2} = -2h_{it}^{-3}\Delta_{h,it} + 6h_{it}^{-4}\Delta_{h,it}^2 - 24h_{it}^{*-5}\Delta_{h,it}^3, \tag{C.53}$$

where $h^*_{it}$ lies between $\tilde{h}_{it,\zeta_0,\tilde{\omega}_i}$ and $h_{it}$. Similar to (C.51), by (C.52)–(C.53), it yields

$$\frac{1}{2NT}\sum_{i=1}^{N}\sum_{t=1}^{T}\Big(\frac{\tilde{u}_{it}^2-\tilde{h}_{it,\zeta_0,\tilde{\omega}_i}}{\tilde{h}_{it,\zeta_0,\tilde{\omega}_i}^2}\frac{\partial \tilde{h}_{it,\zeta_0,\tilde{\omega}_i}}{\partial \tau_l} - \frac{\tilde{u}_{it}^2-\tilde{h}_{it,\zeta_0,\tilde{\omega}_i}}{h_{it}^2}\frac{\partial \tilde{h}_{it,\zeta_0,\tilde{\omega}_i}}{\partial \tau_l}\Big)$$
$$= \frac{1}{2NT}\sum_{i=1}^{N}\sum_{t=1}^{T}(-2\Delta_{h,it})\frac{\tilde{u}_{it}^2-\tilde{h}_{it,\zeta_0,\tilde{\omega}_i}}{h_{it}^3}\frac{\partial \tilde{h}_{it,\zeta_0,\tilde{\omega}_i}}{\partial \tau_l} + o_p\Big(\frac{1}{T}\Big)$$
$$= -\frac{1}{NT}\sum_{i=1}^{N}\sum_{t=1}^{T}(\Delta^{*}_{h,it}+\Delta^{**}_{h,it})\frac{1}{h_{it}^3}\frac{\partial h_{it}}{\partial \tau_l}\Big[u_{it}^2 - h_{it} - \frac{1}{T}\sum_{t=1}^{T}(u_{it}^2-h_{it})\Big] \tag{C.54}$$
$$-\frac{1}{NT}\sum_{i=1}^{N}\sum_{t=1}^{T}(\Delta^{*}_{h,it}+\Delta^{**}_{h,it})h_{it}^{-1}\mathcal{O}^{\sharp}_{23,it,l}\Big(\frac{1}{T}\sum_{t=1}^{T}u_{it}\Big) + o_p\Big(\frac{1}{T}\Big)$$
$$= \frac{1}{NT}(\Delta^{\sharp}_{4,\tau_l}+\Delta^{\flat}_{3,\tau_l}) + o_p\Big(\frac{1}{T}\Big),$$

where

$$\Delta^{\sharp}_{4,\tau_l} = -\sum_{i=1}^{N} \mathrm{E}\Big[\frac{(u_{it}^2 - h_{it})u_{it}c_{it}}{h_{it}^3}\frac{\partial h_{it}}{\partial \tau_l}\Big]$$
$$- \sum_{i=1}^{N} \mathrm{E}(c_{it}h_{it}^{-1}\mathcal{O}^{\sharp}_{23,it,l})\mathrm{E}(u_{it}^2) - \sum_{i=1}^{N} \mathrm{E}(h_{it}^{-1}\mathcal{O}^{\sharp}_{23,it,l})\mathrm{E}[(u_{it}^2 - h_{it})u_{it}].$$

By (C.51) and (C.54), we can get

$$\frac{1}{2NT}\sum_{i=1}^{N}\sum_{t=1}^{T}\Big(\frac{\tilde{u}_{it}^2 - \tilde{h}_{it,\zeta_0,\bar{\omega}_i}}{\tilde{h}_{it,\zeta_0,\bar{\omega}_i}^2}\frac{\partial \tilde{h}_{it,\zeta_0,\bar{\omega}_i}}{\partial \tau_l} - \frac{u_{it}^2 - h_{it,\zeta_0,\bar{\omega}_i}}{h_{it,\zeta_0,\bar{\omega}_i}^2}\frac{\partial h_{it,\zeta_0,\bar{\omega}_i}}{\partial \tau_l}\Big)$$
$$= \frac{1}{2NT}\sum_{i=1}^{N}\sum_{t=1}^{T}\mathrm{E}(\mathcal{O}^{\sharp}_{23,it,l})u_{it} + \frac{1}{NT}(\Delta^{\sharp}_{1,\tau_l} + \Delta^{\sharp}_{2,\tau_l} + \Delta^{\sharp}_{3,\tau_l} + \Delta^{\sharp}_{4,\tau_l}) + o_p\Big(\frac{1}{T}\Big).$$

The above analysis based on $\partial h_{it}/\partial \tau_l$ can be similarly transferred to those for $\partial h_{it}/\partial \nu_k$, with $\Delta^{\sharp}_{c,\nu_k}$ defined in the same way as $\Delta^{\sharp}_{c,\tau_l}$ for $c = 1, 2, 3, 4$. Denote

$$\Delta^{\sharp} = \Delta^{\sharp}_1 + \Delta^{\sharp}_2 + \Delta^{\sharp}_3 + \Delta^{\sharp}_4 \quad \text{with} \quad \Delta^{\sharp}_c = (\Delta^{\sharp}_{c,\tau_1}, ..., \Delta^{\sharp}_{c,\tau_L}, \Delta^{\sharp}_{c,\nu_1}, ..., \Delta^{\sharp}_{c,\nu_K})'. \tag{C.55}$$

Back to (C.47), by (C.55), it follows that

$$\frac{1}{\sqrt{NT}}G^{\sharp} = \frac{1}{2\sqrt{NT}}\sum_{i=1}^{N}\sum_{t=1}^{T}\mathrm{E}(\mathcal{O}^{\sharp}_{23,it})u_{it} + \frac{1}{\sqrt{NT}}\Delta^{\sharp} + o_p\Big(\sqrt{\frac{N}{T}}\Big).$$

It means that the estimation effect of $\mu_0$ causes the asymptotic bias and non-standard asymptotic distribution of $\hat{\zeta}$. □

**Proof for Claim C.9(iv).** As $G^{\flat} = \bar{G} - G$, we have

$$\frac{1}{\sqrt{NT}}G^{\flat} = \frac{1}{2\sqrt{NT}}\sum_{i=1}^{N}\sum_{t=1}^{T}\Big(\frac{u_{it}^2 - h_{it,\zeta_0,\bar{\omega}_i}}{h_{it,\zeta_0,\bar{\omega}_i}^2}\frac{\partial h_{it,\zeta_0,\bar{\omega}_i}}{\partial \zeta} - \frac{u_{it}^2 - h_{it}}{h_{it}^2}\frac{\partial h_{it}}{\partial \zeta}\Big). \tag{C.56}$$

Since $u_{it}^2 - \bar{\omega}_i = u_{it}^2 - \omega_{0i} + \omega_{0i} - \bar{\omega}_i$, it is shown that

$$\begin{aligned}
&\frac{1}{2NT}\sum_{i=1}^{N}\sum_{t=1}^{T}\frac{u_{it}^2 - h_{it,\zeta_0,\bar{\omega}_i}}{h_{it}^2}\frac{\partial h_{it,\zeta_0,\bar{\omega}_i}}{\partial \tau_l} \\
&= \frac{1}{2NT}\sum_{i=1}^{N}\sum_{t=1}^{T}h_{it}^{-2}\Big[\Big(1 - \sum_{k=1}^{K}\nu_{0k}\mathcal{B}^k\Big)^{-1}\Big(1 - \sum_{k=1}^{K}\kappa_{0k}\mathcal{B}^k\Big)(u_{it}^2 - \bar{\omega}_i)\Big] \\
&\quad \times \Big[\Big(1 - \sum_{k=1}^{K}\nu_{0k}\mathcal{B}^k\Big)^{-1}\mathcal{B}^l(u_{it}^2 - \bar{\omega}_i)\Big] \\
&:= \frac{1}{2NT}\sum_{i=1}^{N}\sum_{t=1}^{T}(\mathcal{S}_{1,it} + \mathcal{S}_{2,it}) \times (\mathcal{S}_{3,it,l} + \mathcal{S}_{4,it,l}),
\end{aligned} \tag{C.57}$$

where

$$\mathcal{S}_{1,it} = h_{it}^{-1}\Big[\Big(1-\sum_{k=1}^{K}\nu_{0k}\mathcal{B}^k\Big)^{-1}\Big(1-\sum_{k=1}^{K}\kappa_{0k}\mathcal{B}^k\Big)(u_{it}^2-\omega_{0i})\Big],$$

$$\mathcal{S}_{2,it} = h_{it}^{-1}\Big(1-\sum_{k=1}^{K}\nu_{0k}\Big)^{-1}\Big(1-\sum_{k=1}^{K}\kappa_{0k}\Big)(\omega_{0i}-\bar{\omega}_i),$$

$$\mathcal{S}_{3,it,l} = h_{it}^{-1}\Big[\Big(1-\sum_{k=1}^{K}\nu_{0k}\mathcal{B}^k\Big)^{-1}\mathcal{B}^l(u_{it}^2-\omega_{0i})\Big],$$

$$\mathcal{S}_{4,it,l} = h_{it}^{-1}\Big(1-\sum_{k=1}^{K}\nu_{0k}\Big)^{-1}(\omega_{0i}-\bar{\omega}_i).$$

Below, we analyze $\mathcal{S}_{1,it}\times\mathcal{S}_{3,it,l}$, $\mathcal{S}_{1,it}\times\mathcal{S}_{4,it,l}$, $\mathcal{S}_{2,it}\times\mathcal{S}_{3,it,l}$, and $\mathcal{S}_{2,it}\times\mathcal{S}_{4,it,l}$ one by one.

First, we have

$$\frac{1}{2NT}\sum_{i=1}^{N}\sum_{t=1}^{T}\mathcal{S}_{1,it}\times\mathcal{S}_{3,it,l} = \frac{1}{2NT}\sum_{i=1}^{N}\sum_{t=1}^{T}\frac{u_{it}^2-h_{it}}{h_{it}^2}\frac{\partial h_{it}}{\partial\tau_l}.$$

Second, we can show

$$\begin{aligned}
&\bar{\omega}_i-\omega_{0i}\\
&=\Big(1-\sum_{k=1}^{K}\kappa_{0k}\Big)^{-1}\Big\{\Big(1-\sum_{k=1}^{K}\nu_{0k}\Big)\frac{1}{T}\sum_{t=1}^{T}(u_{it}^2-h_{it})+\sum_{k=1}^{K}\Big(\sum_{k^*=k}^{K}\kappa_{k^*}\Big)\frac{1}{T}(u_{i,1-k}^2-u_{i,T-k+1}^2)\\
&\quad+\sum_{k=1}^{K}\Big(\sum_{k^*=k}^{K}\kappa_{k^*}\Big)\frac{1}{T}(u_{i,T-k+1}^2-h_{i,T-k+1}-u_{i,1-k}+h_{i,1-k}), \qquad \text{(C.58)}
\end{aligned}$$

where only the first item in the RHS of (C.58) has the order $O_p(1/\sqrt{T})$ that is non-negligible. Then, by using a similar argument as for (C.49), we have

$$\begin{aligned}
&\frac{1}{2NT}\sum_{i=1}^{N}\sum_{t=1}^{T}\mathcal{S}_{1,it}\times\mathcal{S}_{4,it,l}\\
&=-\frac{1}{2NT}\sum_{i=1}^{N}\frac{1}{\sqrt{T}}\sum_{t=1}^{T}\frac{u_{it}^2-h_{it}}{h_{it}^2}\Big(\frac{1}{\sqrt{T}}\sum_{t=1}^{T}u_{it}^2-h_{it}\Big)\Big(1-\sum_{k=1}^{K}\kappa_{0k}\Big)^{-1}+o_p\Big(\frac{1}{T}\Big)\\
&=-\frac{1}{2NT}\sum_{i=1}^{N}\mathrm{E}\Big[\frac{(u_{it}^2-h_{it})^2}{h_{it}^2}\Big]\Big(1-\sum_{k=1}^{K}\kappa_{0k}\Big)^{-1}+o_p\Big(\frac{1}{T}\Big)\\
&=\frac{1}{NT}\Delta_{1,\tau_l}^{\flat}+o_p\Big(\frac{1}{T}\Big),
\end{aligned}$$

where the first equation follows from (C.58), and

$$\Delta_{1,\tau_l}^{\flat}=-\frac{1}{2}\sum_{i=1}^{N}[\mathrm{E}(\epsilon_{it}^4)-1]\Big(1-\sum_{k=1}^{K}\kappa_{0k}\Big)^{-1}.$$

Third, we can show

$$\begin{aligned}
&\frac{1}{2NT}\sum_{i=1}^{N}\sum_{t=1}^{T}\mathcal{S}_{2,it}\times\mathcal{S}_{3,it,l}\\
&=-\frac{1}{2NT}\sum_{i=1}^{N}\frac{1}{T}\sum_{t=1}^{T}\frac{1}{h_{it}^2}\frac{\partial h_{it}}{\partial\tau_l}\Big[\sum_{t=1}^{T}(u_{it}^2-h_{it})\Big]\\
&=-\frac{1}{2NT}\sum_{i=1}^{N}\sum_{t=1}^{T}\mathrm{E}\Big(\frac{1}{h_{it}^2}\frac{\partial h_{it}}{\partial\tau_l}\Big)(u_{it}^2-h_{it})+o_p\Big(\frac{1}{T}\Big).
\end{aligned}\tag{C.59}$$

Fourth, it is obtained that

$$\begin{aligned}
&\frac{1}{2NT}\sum_{i=1}^{N}\sum_{t=1}^{T}\mathcal{S}_{2,it}\times\mathcal{S}_{4,it,l}\\
&=\frac{1}{2NT}\sum_{i=1}^{N}\sum_{t=1}^{T}h_{it}^{-2}\Big(1-\sum_{k=1}^{K}\nu_{0k}\Big)^{-2}\Big(1-\sum_{k=1}^{K}\kappa_{0k}\Big)(\omega_{0i}-\bar{\omega}_i)^2\\
&=\frac{1}{2NT}\sum_{i=1}^{N}\frac{1}{T}\sum_{t=1}^{T}h_{it}^{-2}\Big[\frac{1}{\sqrt{T}}\sum_{t=1}^{T}(u_{it}^2-h_{it})\Big]^2\Big(1-\sum_{k=1}^{K}\kappa_{0k}\Big)^{-1}+o_p\Big(\frac{1}{T}\Big)\\
&=\frac{1}{NT}\Delta_{2,\tau_l}^{\flat}+o_p\Big(\frac{1}{T}\Big),
\end{aligned}$$

where

$$\Delta_{2,\tau_l}^{\flat}=\frac{1}{2}\sum_{i=1}^{N}\mathrm{E}(h_{it}^{-2})\mathrm{E}(h_{it}^2)[\mathrm{E}(\epsilon_{it}^4)-1]\Big(1-\sum_{k=1}^{K}\kappa_{0k}\Big)^{-1}.$$

By (C.57), it follows that

$$\begin{aligned}
&\frac{1}{2NT}\sum_{i=1}^{N}\sum_{t=1}^{T}\Big(\frac{u_{it}^2-h_{it,\zeta_0,\bar{\omega}_i}}{h_{it}^2}\frac{\partial h_{it,\zeta_0,\bar{\omega}_i}}{\partial\tau_l}-\frac{u_{it}^2-h_{it}}{h_{it}^2}\frac{\partial h_{it}}{\partial\tau_l}\Big)\\
&=-\frac{1}{2NT}\sum_{i=1}^{N}\sum_{t=1}^{T}\mathrm{E}\Big(\frac{1}{h_{it}^2}\frac{\partial h_{it}}{\partial\tau_l}\Big)(u_{it}^2-h_{it})+\frac{1}{NT}(\Delta_{1,\tau_l}^{\flat}+\Delta_{2,\tau_l}^{\flat})+o_p\Big(\frac{1}{T}\Big).
\end{aligned}\tag{C.60}$$

Next, recall $\Delta_{h,it}^{**}=T^{-1}\sum_{t=1}^{T}(u_{it}^2-h_{it})$ and

$$\Delta_{3,\tau_l}^{\flat}=-\sum_{i=1}^{N}\Big[\mathrm{E}\Big(\frac{1}{h_{it}}\frac{\partial h_{it}}{\partial\tau_l}\Big)-\mathrm{E}\Big(\frac{1}{h_{it}^3}\frac{\partial h_{it}}{\partial\tau_l}\Big)\mathrm{E}(h_{it}^2)\Big][\mathrm{E}(\epsilon_{it}^4)-1].$$

Then, similar to (C.53)–(C.54), we can show

$$\begin{aligned}
&\frac{1}{2NT}\sum_{i=1}^{N}\sum_{t=1}^{T}\Big(\frac{u_{it}^2-h_{it,\zeta_0,\bar{\omega}_i}}{h_{it,\zeta_0,\bar{\omega}_i}^2}\frac{\partial h_{it,\zeta_0,\bar{\omega}_i}}{\partial\tau_l}-\frac{u_{it}^2-h_{it,\zeta_0,\bar{\omega}_i}}{h_{it}^2}\frac{\partial h_{it,\zeta_0,\bar{\omega}_i}}{\partial\tau_l}\Big)\\
&=\frac{1}{2NT}\sum_{i=1}^{N}\sum_{t=1}^{T}(-2\Delta_{h,it}^{**})\frac{u_{it}^2-h_{it,\zeta_0,\bar{\omega}_i}}{h_{it}^3}\frac{\partial h_{it,\zeta_0,\bar{\omega}_i}}{\partial\tau_l}+o_p\Big(\frac{1}{T}\Big)\\
&=-\frac{1}{NT}\sum_{i=1}^{N}\frac{1}{\sqrt{T}}\sum_{t=1}^{T}\frac{u_{it}^2-h_{it}}{h_{it}^3}\frac{\partial h_{it}}{\partial\tau_l}\Big[\frac{1}{\sqrt{T}}\sum_{t=1}^{T}(u_{it}^2-h_{it})\Big]\\
&\quad+\frac{1}{NT}\sum_{i=1}^{N}\frac{1}{T}\sum_{t=1}^{T}\frac{1}{h_{it}^3}\frac{\partial h_{it}}{\partial\tau_l}\Big[\frac{1}{\sqrt{T}}\sum_{t=1}^{T}(u_{it}^2-h_{it})\Big]^2+o_p\Big(\frac{1}{T}\Big)\\
&=\frac{1}{NT}\Delta_{3,\tau_l}^{\flat}+o_p\Big(\frac{1}{T}\Big),
\end{aligned}\tag{C.61}$$

where the first equation follows from (C.39), the second equation is caused by (C.59), and the third equation shares the same idea as for (C.49).

By (C.60)–(C.61), we can get

$$\begin{aligned}
&\frac{1}{2NT}\sum_{i=1}^{N}\sum_{t=1}^{T}\Big(\frac{u_{it}^2-h_{it,\zeta_0,\bar{\omega}_i}}{h_{it,\zeta_0,\bar{\omega}_i}^2}\frac{\partial h_{it,\zeta_0,\bar{\omega}_i}}{\partial\tau_l}-\frac{u_{it}^2-h_{it}}{h_{it}^2}\frac{\partial h_{it}}{\partial\tau_l}\Big)\\
&=-\frac{1}{2NT}\sum_{i=1}^{N}\sum_{t=1}^{T}\mathrm{E}\Big(\frac{1}{h_{it}^2}\frac{\partial h_{it}}{\partial\tau_l}\Big)(u_{it}^2-h_{it})+\frac{1}{NT}(\Delta_{1,\tau_l}^{\flat}+\Delta_{2,\tau_l}^{\flat}+\Delta_{3,\tau_l}^{\flat})+o_p\Big(\frac{1}{T}\Big).
\end{aligned}$$

The above analysis based on $\partial h_{it}/\partial\tau_l$ can be similarly transferred to those for $\partial h_{it}/\partial\nu_k$, with $\Delta_{c,\nu_k}^{\flat}$ defined in the same way as $\Delta_{c,\tau_l}^{\flat}$ for $c=1,2,3$. Denote

$$\Delta^{\flat}=\Delta_1^{\flat}+\Delta_2^{\flat}+\Delta_3^{\flat}\quad\text{with}\quad\Delta_c^{\flat}=(\Delta_{c,\tau_1}^{\flat},...,\Delta_{c,\tau_L}^{\flat},\Delta_{c,\nu_1}^{\flat},...,\Delta_{c,\nu_K}^{\flat})'.\tag{C.62}$$

Back to (C.56), it follows that

$$\frac{1}{\sqrt{NT}}G^{\flat}=-\frac{1}{2NT}\sum_{i=1}^{N}\sum_{t=1}^{T}\mathrm{E}\Big(\frac{1}{h_{it}^2}\frac{\partial h_{it}}{\partial\zeta}\Big)(u_{it}^2-h_{it})+\frac{1}{\sqrt{NT}}\Delta^{\flat}+o_p\Big(\sqrt{\frac{N}{T}}\Big).$$

It shows that the estimation effect of $\omega_0$ causes the asymptotic bias and non-standard asymptotic distribution of $\hat{\zeta}$. □

**Proof for Theorem 4.4.** First, we consider the consistency of $\hat{\zeta}$. Following Francq and Zakoïan (2004) and Francq et al. (2011), it is not difficult to show that $\hat{\zeta}^0-\zeta_0=o_p(1)$, where $\hat{\zeta}^0=\arg\max L_{\zeta,\omega_0}$. Note that

$$\frac{1}{NT}\hat{L}_{\zeta,\hat{\omega}}-\frac{1}{NT}L_{\zeta,\omega_0}=\frac{1}{NT}L_{\zeta}^{\dagger}+\frac{1}{NT}L_{\zeta}^{\S}+\frac{1}{NT}L_{\zeta}^{\sharp}+\frac{1}{NT}L_{\zeta}^{\flat}.$$

Then, by Lemma C.8 we have

$$\frac{1}{NT}\hat{L}_{\zeta,\hat{\omega}} - \frac{1}{NT}L_{\zeta,\omega_0} = o_p(1),$$

entailing that $\hat{\zeta} - \hat{\zeta}^0 = o_p(1)$. Hence, it follows that $\hat{\zeta} - \zeta_0 = o_p(1)$.

Next, we study the asymptotic distribution of $\hat{\zeta}$. By Taylor's expansion, we have

$$\sqrt{NT}(\hat{\zeta} - \zeta_0) = \frac{1}{\sqrt{NT}}\Gamma_2^{*-1}\hat{G} = \frac{1}{\sqrt{NT}}\Gamma_2^{*-1}(G + G^{\dagger} + G^{\S} + G^{\sharp} + G^{\flat}), \tag{C.63}$$

where $\Gamma_2^*$ is a $(L+K)\times(L+K)$–dimensional matrix with $(i,j)$-th entry $\gamma_{2,ij} = -(NT)^{-1}$ $\partial^2\hat{L}_{\zeta_{ij}^*,\hat{\omega}}/\partial\zeta_i\partial\zeta_j$, and $\zeta_{ij}^* \in \Theta_\zeta$ lies between $\hat{\zeta}$ and $\zeta_0$. $\hat{G} = \partial\hat{L}_{\zeta,\hat{\omega}}/\partial\zeta\big|_{\zeta=\zeta_0}$, and $G$, $G^{\dagger}$, $G^{\S}$, $G^{\sharp}$, and $G^{\flat}$ are defined in (4.5)–(4.8).

For $\hat{W} = \partial^2\hat{L}_{\zeta,\hat{\omega}}/\partial\zeta\partial\zeta'\big|_{\zeta=\zeta_0}$, similar to Claims C.8–C.9, we can show

$$\frac{1}{NT}\hat{W} = \Gamma_2 + O_p\Big(\sqrt{\frac{1}{T}}\Big) = O_p(1) + O_p\Big(\sqrt{\frac{1}{T}}\Big).$$

Like (C.21), we have

$$\Gamma_2^* = \Gamma_2 + O_p\Big(\sqrt{\frac{1}{T}}\Big). \tag{C.64}$$

Moreover, in view of (B.6) and $h_{it} = h_{it,\zeta_0,\omega_0}$, we know

$$\frac{1}{\sqrt{NT}}G = \frac{1}{\sqrt{NT}}\sum_{i=1}^{N}\sum_{t=1}^{T}\frac{1}{2h_{it}^2}\frac{\partial h_{it}}{\partial\zeta}(u_{it}^2 - h_{it}). \tag{C.65}$$

Hence, by (C.63)–(C.65) and Lemmas C.6 and C.9, the desirable result follows. □

**Proof for Theorem 4.5.** By (C.22), (C.31), (C.37), and (C.58), it is not hard to show

$$\begin{aligned}
&\hat{\omega}_i - \omega_{0i}\\
&= \hat{\omega}_i - \check{\omega}_i + \check{\omega}_i - \tilde{\omega}_i + \tilde{\omega}_i - \bar{\omega}_i + \bar{\omega}_i - \omega_{0i}\\
&= \Big(1 - \sum_{k=1}^{K}\kappa_{0k}\Big)^{-1}\Big(1 - \sum_{k=1}^{K}\nu_{0k}\Big)\frac{1}{T}\sum_{t=1}^{T}(u_{it}^2 - h_{it}) + o_p\Big(\sqrt{\frac{1}{T}}\Big).
\end{aligned}$$

Then, the desirable result in Theorem 4.5 can be obtained directly. □

**Proof for Theorem 4.6.** Since the proof is similar to that for Theorem 4.3, the related details are omitted. □

# References


Amemiya, T. (1985). *Advanced Econometrics*. Cambridge: Harvard University Press.

Bishop, Y. M., Fienberg, S. E., and Holland, P. W. (2007). *Discrete Multivariate Analysis: Theory and Practice*. New York: Springer Science & Business Media.

Bühlmann, P. (1995). Moving-average representation of autoregressive approximations. *Stochastic Processes and Their Applications* **60**, 331–342.

Chung, K. L. (2001). *A Course in Probability Theory*. New York: Academic Press.

Dalla, V., Giraitis, L., and Koul, H. L. (2014). Studentizing weighted sums of linear processes. *Journal of Time Series Analysis* **35**, 151–172.

Francq, C., Horváth, L., and Zakoïan, J. M. (2011). Merits and drawbacks of variance targeting in GARCH models. *Journal of Financial Econometrics* **9**, 619–656.

Francq, C. and Zakoïan, J. M. (2004). Maximum likelihood estimation of pure GARCH and ARMA-GARCH processes. *Bernoulli* **10**, 605–637.

Giraitis, L., Taniguchi, M., and Taqqu, M. S. (2017). Asymptotic normality of quadratic forms of martingale differences. *Statistical Inference for Stochastic Processes* **20**, 315–327.

Hall, P. and Heyde, C. C. (1980). *Martingale Limit Theory and its Application*. New York: Academic Press.

Ling, S. (2007). Self-weighted and local quasi-maximum likelihood estimators for ARMA-GARCH/IGARCH models. *Journal of Econometrics* **140**, 849–873.

Phillips, P. C. and Moon, H. R. (1999). Linear regression limit theory for nonstationary panel data. *Econometrica* **67**, 1057–1111.

Stout, W. F. (1974). *Almost Sure Convergence*. New York: Academic Press.
